# Supplementary material for: Test for mean matrix in GMANOVA model under heteroscedasticity and non-normality for high-dimensional data
Source: arXiv:2008.04692 ancillary file (2020-08-12)
Supplement: Supplementary file 1 [file supplimentaly.pdf]

# Supplement to "Test for mean matrix in GMANOVA model under heteroscedaticity and non-normality for high-dimensional data"


Takayuki Yamada*

*Department of Mathematical Sciences,*
*Shimane University,*
*1060 Nishikawatsu-cho, Matsue, Shimane 690-8504, Japan*

Tetsuto Himeno

*Faculty of Data Science,*
*Shiga University,*
*1-1-1 Banba, Hikone, Shiga 522-8522, Japan*

Annika Tillander

*Department of Computer and Information Science,*
*Linköping University,*
*581 83 Linköping, Sweden*

Tatjana Pavlenko

*Department of Mathematics,*
*KTH Royal Institute of Technology,*
*SE-100 44 Stockholm, Sweden*



## Abstract

In this supplement we prove Lemma 2 and Lemma 4-6. In addition, specific results contained in the proposed class of tests are reviewed, and the results of numerical evaluations conducted through various finite-sample simulation scenarios, along with an example using real data are also reported.



*Keywords:* Asymptotic distribution, GMANOVA model, Bilateral linear hypothesis on mean matrix, High-dimensional data, Bias correction approach, Non-normal model, $(N, p)$-asymptotic.
*AMS 2000 subject classification*: Primary 62H15, Secondary 62H10


## S1. Outline of supplemental material and preliminary

This supplement is constructed as follows. In Section S2, we provide the proof of Lemma 2. In Section S3, we prove Lemma 4-6. We review specific results contained in the proposed class of tests in Section S4. In Section S5, we report the results of numerical evaluations conducted through various finite-sample simulation scenarios, along with an example using real data.


*Corresponding author
*Email address:* `takayuki-yamada@riko.shimane-u.ac.jp` (Takayuki Yamada)

To being the notation simplicity, we use the notation $\sum_{i_1,\ldots,i_k}^{N}$ as the sum for all of different indices $\{i_1,\ldots,i_k\}$. For example, $\sum_{i,j,k}^{N} = \sum_{i=1}^{N}\sum_{\substack{j=1\\ j\neq i}}^{N}\sum_{\substack{k=1\\ k\neq i,k\neq j}}^{N}$.

## S2. Proof of Lemma 2

We prove the unbiasedness for $\hat{a}_{i,2}$. For making presentation simple, instead of considering under the model (1), we consider under the following multivariate linear model for $N\times p$ observation matrix $\boldsymbol{Y}$ which is obtained by independently observing a $p$-dimensional variate $\boldsymbol{y}$ for $N$ subjects, i.e. $\boldsymbol{Y} = (\boldsymbol{y}_1,\ldots,\boldsymbol{y}_N)'$, where $\boldsymbol{y}_1, \ldots, \boldsymbol{y}_N$ are independent $p$-dimensional random vectors:

$$\boldsymbol{Y} = \boldsymbol{A}\boldsymbol{\Theta} + \boldsymbol{Z}\boldsymbol{\Sigma}^{1/2},$$

where $\boldsymbol{A}$ is known $N\times k$ design matrix with the lank $k$, $\boldsymbol{\Theta}$ is a $k\times p$ unknown parameter matrix, $\boldsymbol{Z} = (\boldsymbol{z}_1,\ldots,\boldsymbol{z}_N)'$ is an $N\times p$ error matrix whose rows are independently and identically distributed as a $p$-dimensional distribution with mean $\boldsymbol{0}$ and covariance matrix $\boldsymbol{I}_p$, and $\boldsymbol{\Sigma}$ is a $p\times p$ covariance matrix of $\boldsymbol{y}$ and $\boldsymbol{\Sigma}^{1/2}$ is a square root of $\boldsymbol{\Sigma}$. Let $a_i = \mathrm{tr}(\boldsymbol{\Sigma}^i)$ for $i=1,2$, and $\kappa = E[(\boldsymbol{z}'\boldsymbol{\Sigma}\boldsymbol{z})^2] - 2\mathrm{tr}(\boldsymbol{\Sigma}^2) - (\mathrm{tr}(\boldsymbol{\Sigma}))^2$.

**Lemma 9.** *The unbiased estimators for $a_2$, $a_1^2$ and $\kappa$ are expressed as follows:*

$$\begin{aligned}
\hat{a}_2 &= \frac{1}{(N-k)\tau_3}\left[\left\{(N-k)^2\tau_2 - \tau_1^2\right\}\mathrm{tr}(\boldsymbol{S}^2) - \left\{\{(N-k)\tau_2 - \tau_1^2\right\}(\mathrm{tr}(\boldsymbol{S}))^2 - (N-k-1)\tau_1 Q\right],\\
\widehat{a_1^2} &= \frac{1}{(N-k)\tau_3}\left[-2\{(N-k)\tau_2 - \tau_1^2\}\mathrm{tr}(\boldsymbol{S}^2) + \{(N-k+1)(N-k)\tau_2 - 2\tau_1^2\}(\mathrm{tr}(\boldsymbol{S}))^2\right.\\
&\quad \left. -(N-k-1)\tau_1 Q\right],\\
\hat{\kappa} &= \frac{N-k-1}{\tau_3}\left[-2\tau_1\mathrm{tr}(\boldsymbol{S}^2) - \tau_1(\mathrm{tr}(\boldsymbol{S}))^2 + (N-k+2)Q\right],
\end{aligned}$$

*where*

$$\tau_i = \mathrm{tr}\left(((\boldsymbol{I}_N - \boldsymbol{\Pi}_{\boldsymbol{A}})\odot(\boldsymbol{I}_N - \boldsymbol{\Pi}_{\boldsymbol{A}}))^i\right), \quad i=1,2, \quad \tau_3 = \frac{N-k-1}{(N-k)^2}\left\{(N-k)(N-k+2)\tau_2 - 3\tau_1^2\right\},$$

*$\boldsymbol{\Pi}_{\boldsymbol{A}} = \boldsymbol{A}(\boldsymbol{A}'\boldsymbol{A})^{+}\boldsymbol{A}'$, the symbol "$\boldsymbol{A}^{+}$" denotes the Moore-Penrose inverse matrix of $\boldsymbol{A}$, the symbol "$\odot$" denotes the Hadamard product of matrices;*

$$\begin{aligned}
\boldsymbol{S} &= \frac{1}{N-k}\boldsymbol{Y}'(\boldsymbol{I}_N - \boldsymbol{\Pi}_{\boldsymbol{A}})\boldsymbol{Y};\\
Q &= \frac{1}{N-k}\sum_{i=1}^{N}\{(\boldsymbol{y}_i - \hat{\boldsymbol{y}}_i)'(\boldsymbol{y}_i - \hat{\boldsymbol{y}}_i)\}^2, \quad (\hat{\boldsymbol{y}}_1,\ldots,\hat{\boldsymbol{y}}_N)' = \boldsymbol{\Pi}_{\boldsymbol{A}}(\boldsymbol{y}_1,\ldots,\boldsymbol{y}_N)' = \boldsymbol{\Pi}_{\boldsymbol{A}}\boldsymbol{Y}.
\end{aligned}$$

The unbiasedness of $\hat{a}_{i,2}$ in Lemma 2 is followed from the ones of $\hat{a}_2$ in Lemma 9 by replacing $N$, $\boldsymbol{Y}$, $\boldsymbol{A}$, $\boldsymbol{\Theta}$ and $\boldsymbol{\Sigma}$ with $N_i$, $\boldsymbol{X}_i$, $\boldsymbol{A}_i$, $\boldsymbol{\Theta}\boldsymbol{B}$ and $\boldsymbol{\mathcal{P}}\boldsymbol{\Sigma}_i\boldsymbol{\mathcal{P}}'$, respectively.

*Proof of Lemma 9.* It can be expressed that $\boldsymbol{S} = (N-k)^{-1}\boldsymbol{\Sigma}^{1/2}\boldsymbol{Z}'(\boldsymbol{I}_N - \boldsymbol{\Pi}_{\boldsymbol{A}})\boldsymbol{Z}\boldsymbol{\Sigma}^{1/2}$, and thus is

described that

$$\begin{aligned}
\mathrm{tr}(\boldsymbol{S}) &= \frac{1}{N-k}\mathrm{tr}\left((\boldsymbol{I}_N - \boldsymbol{\Pi}_{\boldsymbol{A}})\boldsymbol{Z}\boldsymbol{\Sigma}\boldsymbol{Z}'\right) = \frac{1}{N-k}\left(\sum_{i=1}^N q_{ii}\boldsymbol{z}_i'\boldsymbol{\Sigma}\boldsymbol{z}_i + \sum_{i,j}^N q_{ij}\boldsymbol{z}_i'\boldsymbol{\Sigma}\boldsymbol{z}_j\right), \\
\mathrm{tr}(\boldsymbol{S}^2) &= \frac{1}{(N-k)^2}\mathrm{tr}\left((\boldsymbol{I}_N - \boldsymbol{\Pi}_{\boldsymbol{A}})\boldsymbol{Z}\boldsymbol{\Sigma}\boldsymbol{Z}'\right)^2 = \frac{1}{(N-k)^2}\left(\sum_{i=1}^N\sum_{j=1}^N\sum_{k=1}^N\sum_{\ell=1}^N q_{ij}\boldsymbol{z}_j'\boldsymbol{\Sigma}\boldsymbol{z}_k q_{k\ell}\boldsymbol{z}_\ell'\boldsymbol{\Sigma}\boldsymbol{z}_i\right), \\
Q &= \frac{1}{N-k}\mathrm{tr}\left(\left\{(\boldsymbol{I}_N - \boldsymbol{\Pi}_{\boldsymbol{A}})\boldsymbol{Z}\boldsymbol{\Sigma}\boldsymbol{Z}'(\boldsymbol{I}_N - \boldsymbol{\Pi}_{\boldsymbol{A}})\right\} \odot \left\{(\boldsymbol{I}_N - \boldsymbol{\Pi}_{\boldsymbol{A}})\boldsymbol{Z}\boldsymbol{\Sigma}\boldsymbol{Z}'(\boldsymbol{I}_N - \boldsymbol{\Pi}_{\boldsymbol{A}})\right\}\right) \\
&= \sum_{i=1}^N\left(\sum_{j=1}^N\sum_{k=1}^N q_{ij}\boldsymbol{z}_j'\boldsymbol{\Sigma}\boldsymbol{z}_k q_{ki}\right)^2,
\end{aligned}$$

where $(q_{ij}) = \boldsymbol{I}_N - \boldsymbol{\Pi}_{\boldsymbol{A}}$. Then, we have

$$\begin{aligned}
(\mathrm{tr}(\boldsymbol{S}))^2 &= \frac{1}{(N-k)^2}\left(\sum_{i=1}^N q_{ii}\boldsymbol{z}_i'\boldsymbol{\Sigma}\boldsymbol{z}_i + \sum_{i,j}^N q_{ij}\boldsymbol{z}_i'\boldsymbol{\Sigma}\boldsymbol{z}_j\right)^2 \\
&= \frac{1}{(N-k)^2}\left(\sum_{i=1}^N q_{ii}^2(\boldsymbol{z}_i'\boldsymbol{\Sigma}\boldsymbol{z}_i)^2 + \sum_{i,j}^N q_{ii}q_{jj}\boldsymbol{z}_i'\boldsymbol{\Sigma}\boldsymbol{z}_i\boldsymbol{z}_j'\boldsymbol{\Sigma}\boldsymbol{z}_j + 2\sum_{i,j}^N q_{ij}^2(\boldsymbol{z}_i'\boldsymbol{\Sigma}\boldsymbol{z}_j)^2\right. \\
&\quad + 4\sum_{i,j}^N q_{ii}q_{ij}\boldsymbol{z}_i'\boldsymbol{\Sigma}\boldsymbol{z}_i\boldsymbol{z}_i'\boldsymbol{\Sigma}\boldsymbol{z}_j + 2\sum_{i,j,k}^N q_{ii}q_{jk}\boldsymbol{z}_i'\boldsymbol{\Sigma}\boldsymbol{z}_i\boldsymbol{z}_j'\boldsymbol{\Sigma}\boldsymbol{z}_k + 4\sum_{i,j,k}^N q_{ij}q_{ik}\boldsymbol{z}_i'\boldsymbol{\Sigma}\boldsymbol{z}_j\boldsymbol{z}_i'\boldsymbol{\Sigma}\boldsymbol{z}_k \\
&\quad \left. + \sum_{i,j,k,\ell}^N q_{ij}q_{k\ell}\boldsymbol{z}_i'\boldsymbol{\Sigma}\boldsymbol{z}_j\boldsymbol{z}_k'\boldsymbol{\Sigma}\boldsymbol{z}_\ell\right), \\
\mathrm{tr}(\boldsymbol{S}^2) &= \frac{1}{(N-k)^2}\left(\sum_{i=1}^N q_{ii}^2(\boldsymbol{z}_i'\boldsymbol{\Sigma}\boldsymbol{z}_i)^2 + \sum_{i,j}^N q_{ij}^2\boldsymbol{z}_i'\boldsymbol{\Sigma}\boldsymbol{z}_i\boldsymbol{z}_j'\boldsymbol{\Sigma}\boldsymbol{z}_j + \sum_{i,j}^N (q_{ii}q_{jj} + q_{ij}^2)(\boldsymbol{z}_i'\boldsymbol{\Sigma}\boldsymbol{z}_j)^2\right. \\
&\quad + 4\sum_{i,j}^N q_{ii}q_{ij}\boldsymbol{z}_i'\boldsymbol{\Sigma}\boldsymbol{z}_i\boldsymbol{z}_i'\boldsymbol{\Sigma}\boldsymbol{z}_j + 2\sum_{i,j,k}^N q_{ij}q_{ik}\boldsymbol{z}_i'\boldsymbol{\Sigma}\boldsymbol{z}_i\boldsymbol{z}_j'\boldsymbol{\Sigma}\boldsymbol{z}_k \\
&\quad \left. + 2\sum_{i,j,k}^N (q_{ii}q_{jk} + q_{ij}q_{ik})\boldsymbol{z}_i'\boldsymbol{\Sigma}\boldsymbol{z}_j\boldsymbol{z}_i'\boldsymbol{\Sigma}\boldsymbol{z}_k + \sum_{i,j,k,\ell}^N q_{ik}q_{j\ell}\boldsymbol{z}_i'\boldsymbol{\Sigma}\boldsymbol{z}_j\boldsymbol{z}_k'\boldsymbol{\Sigma}\boldsymbol{z}_\ell\right), \\
Q &= \frac{1}{N-k}\sum_{i=1}^N\left(\sum_{j=1}^N q_{ij}^2\boldsymbol{z}_j'\boldsymbol{\Sigma}\boldsymbol{z}_j + \sum_{j,k}^N q_{ij}q_{ik}\boldsymbol{z}_j'\boldsymbol{\Sigma}\boldsymbol{z}_k\right)^2 \\
&= \frac{1}{N-k}\left\{\sum_{i=1}^N\left(\sum_{j=1}^N q_{ij}^4\right)(\boldsymbol{z}_i'\boldsymbol{\Sigma}\boldsymbol{z}_i)^2 + \sum_{i,j}^N\left(\sum_{k=1}^N q_{ik}^2q_{jk}^2\right)\boldsymbol{z}_i'\boldsymbol{\Sigma}\boldsymbol{z}_i\boldsymbol{z}_j'\boldsymbol{\Sigma}\boldsymbol{z}_j\right.
\end{aligned}$$

$$+ 2\sum_{i,j}^{N}\left(\sum_{k=1}^{N} q_{ik}^2 q_{jk}^2\right)(\boldsymbol{z}_i'\boldsymbol{\Sigma}\boldsymbol{z}_j)^2 + 4\sum_{i,j}^{N}\left(\sum_{k=1}^{N} q_{ik}^3 q_{jk}\right)\boldsymbol{z}_i'\boldsymbol{\Sigma}\boldsymbol{z}_i\boldsymbol{z}_i'\boldsymbol{\Sigma}\boldsymbol{z}_j$$
$$+ 2\sum_{i,j,k}^{N}\left(\sum_{\ell=1}^{N} q_{i\ell}^2 q_{j\ell} q_{k\ell}\right)\boldsymbol{z}_i'\boldsymbol{\Sigma}\boldsymbol{z}_i\boldsymbol{z}_j'\boldsymbol{\Sigma}\boldsymbol{z}_k + 4\sum_{i,j,k}^{N}\left(\sum_{\ell=1}^{N} q_{i\ell}^2 q_{j\ell} q_{k\ell}\right)\boldsymbol{z}_i'\boldsymbol{\Sigma}\boldsymbol{z}_j\boldsymbol{z}_i'\boldsymbol{\Sigma}\boldsymbol{z}_k$$
$$\left. + \sum_{i,j,k,\ell}^{N}\left(\sum_{\alpha=1}^{N} q_{i\alpha} q_{j\alpha} q_{k\alpha} q_{\ell\alpha}\right)\boldsymbol{z}_i'\boldsymbol{\Sigma}\boldsymbol{z}_j\boldsymbol{z}_k'\boldsymbol{\Sigma}\boldsymbol{z}_\ell \right\}.$$

These expectations can be described as follows:

$$\begin{aligned}
E\left[\mathrm{tr}(\boldsymbol{S}^2)\right] &= \frac{1}{(N-k)^2}\tau_1\kappa + \frac{N-k+1}{N-k}a_2 + \frac{1}{N-k}a_1^2, \\
E\left[(\mathrm{tr}(\boldsymbol{S}))^2\right] &= \frac{1}{(N-k)^2}\tau_1\kappa + \frac{2}{N-k}a_2 + a_1^2, \\
E[Q] &= \frac{1}{N-k}\tau_2\kappa + \frac{2}{N-k}\tau_1 a_2 + \frac{1}{N-k}\tau_1 a_1^2.
\end{aligned}$$

By solving this system of linear equations in terms of $\kappa$, $a_2$ and $a_1^2$, we can obtain the unique solutions as follows:

$$\begin{aligned}
a_2 &= \frac{1}{(N-k)\tau_3}E\left[\left\{(N-k)^2\tau_2 - \tau_1^2\right\}\mathrm{tr}(\boldsymbol{S}^2) - \left\{\left\{(N-k)\tau_2 - \tau_1^2\right\}(\mathrm{tr}(\boldsymbol{S}))^2 - (N-k-1)\tau_1 Q\right], \\
a_1^2 &= \frac{1}{(N-k)\tau_3}E\left[-2\{(N-k)\tau_2 - \tau_1^2\}\mathrm{tr}(\boldsymbol{S}^2) + \{(N-k+1)(N-k)\tau_2 - 2\tau_1^2\}(\mathrm{tr}(\boldsymbol{S}))^2\right. \\
&\quad \left. -(N-k-1)\tau_1 Q\right], \\
\kappa &= \frac{N-k-1}{\tau_3}E\left[-2\tau_1\mathrm{tr}(\boldsymbol{S}^2) - \tau_1(\mathrm{tr}(\boldsymbol{S}))^2 + (N-k+2)Q\right].
\end{aligned}$$

Unbiased estimators are obtained from these formulae. □

## S3. Proofs of Lemma 4-6

In this section, we give proofs of Lemma 4-6. We use the notations defined in the original papers given as follows:

$$\boldsymbol{\Psi}_i = \boldsymbol{\mathcal{P}}\boldsymbol{\Sigma}_i\boldsymbol{\mathcal{P}}', \quad \boldsymbol{\Upsilon}_i = \boldsymbol{\mathcal{P}}\boldsymbol{\Sigma}_i^{1/2}.$$

Define

$$(p_{ij}) = \boldsymbol{\Pi}_{\boldsymbol{A}_1} = \boldsymbol{A}_1(\boldsymbol{A}_1'\boldsymbol{A}_1)^{+}\boldsymbol{A}_1'.$$

and

$$\mathfrak{q} = E[(\boldsymbol{z}'\bar{\boldsymbol{\Upsilon}}_1'\bar{\boldsymbol{\Upsilon}}_1\boldsymbol{z})^2].$$

It follows from Lemma 3 that

$$\frac{\mathfrak{q}}{(\mathrm{tr}(\boldsymbol{\Psi}_1))^2} = \frac{E[(\boldsymbol{z}'\bar{\boldsymbol{\Upsilon}}_1'\bar{\boldsymbol{\Upsilon}}_1\boldsymbol{z})^2]}{(\mathrm{tr}(\boldsymbol{\Psi}_1))^2} = O(1) \quad (p \to \infty).$$

Suppose that the notation "$\odot^i \boldsymbol{A}$" represents the Hadamard product of $i$ matrices positive semi-definite symmetric matrix $\boldsymbol{A}$, i.e.,

$$\odot^i \boldsymbol{A} = \boldsymbol{A} \odot \boldsymbol{A} \odot \cdots \odot \boldsymbol{A}, \quad (i \text{ times}).$$

We note that $\odot^i \boldsymbol{A}$ is positive semi-definite symmetric matrix, which is guaranteed by Schur's product theorem (cf. Schott [5]).

*S3.1. Proof of Lemma* 4

Firstly, we give a lemma which is used to prove Lemma 4.

**Lemma 10.** *It holds that*

(i) $N_1 - k_1 - \tau_{1,1}^2/\tau_{1,2} = O(1)$ *as* $N_1 \to \infty$.
(ii) $1 - \tau_{1,1}/\tau_{1,2} = O(N_1^{-1})$ *as* $N_1 \to \infty$.

*Proof of Lemma 10.* It can be expressed that

$$\tau_{1,i} = (N_1 - k_1)\left\{1 + \frac{1}{N_1 - k_1}R_i\right\}, \quad i = 1, 2,$$

where

$$R_1 = \sum_{i=1}^{N_1} p_{ii}^2 - k_1,$$
$$R_2 = -3k + 6\sum_{i=1}^{N_1} p_{ii}^2 + \sum_{i=1}^{N_1}(p_{ii}^4 - 4p_{ii}^3) + \sum_{i,j}^{N_1} p_{ij}^4.$$

Since $\boldsymbol{\Pi}_{\boldsymbol{A}_1}$ is proportional matrix, it holds that $0 \le p_{ii} \le 1$, $i = 1, \ldots, N_1$; and also holds that $0 \le p_{ij}^2 \le 1$, $i, j = 1, \ldots, N_1, i \ne j$; and thus the following inequalities can be established:

$$0 \le \sum_{i=1}^{N_1} p_{ii}^{\ell} \le \sum_{i=1}^{N_1} p_{ii} = \mathrm{tr}(\boldsymbol{\Pi}_{\boldsymbol{A}_1}) \le k_1, \quad \ell = 2, 3, 4, \tag{13}$$

$$0 \le \sum_{i,j}^{N_1} p_{ij}^4 \le \sum_{i,j}^{N_1} p_{ij}^2 \le \sum_{i=1}^{N_1}\sum_{j=1}^{N_1} p_{ij}^2 = \mathrm{tr}(\boldsymbol{\Pi}_{\boldsymbol{A}_1}^2) = \mathrm{tr}(\boldsymbol{\Pi}_{\boldsymbol{A}_1}) \le k_1. \tag{14}$$

From them we find that $R_i = O(1)$ as $N_1 \to \infty$ for $i = 1, 2$. Thus,

$$\begin{aligned}
N_1 - k_1 - \frac{\tau_{1,1}^2}{\tau_{1,2}} &= (N_1 - k_1) - (N_1 - k_1)\frac{\{1 + R_1/(N_1 - k_1)\}^2}{1 + R_2/(N_1 - k_1)} \\
&= (N_1 - k_1) - (N_1 - k_1)\left[1 + \frac{\{R_1/(N_1 - k_1)\}^2 + 2R_1/(N_1 - k_1) - R_2/(N_1 - k_1)}{1 + R_2/(N_1 - k_1)}\right] \\
&= \frac{R_1^2/(N_1 - k_1) + 2R_1 - R_2}{1 + R_2/(N_1 - k_1)} = O(1), \\
1 - \frac{\tau_{1,1}}{\tau_{1,2}} &= 1 - \frac{(N_1 - k_1)\left\{1 + \dfrac{R_1}{N_1 - k_1}\right\}}{(N_1 - k_1)\left\{1 + \dfrac{R_2}{N_1 - k_1}\right\}} \\
&= 1 - \frac{1 + \dfrac{R_2}{N_1 - k_1} + \left(\dfrac{R_1}{N_1 - k_1} - \dfrac{R_2}{N_1 - k_1}\right)}{1 + \dfrac{R_2}{N_1 - k_1}} \\
&= \frac{1}{N_1 - k_1}\frac{R_2 - R_1}{1 + \dfrac{R_2}{N_1 - k_1}} = O(N_1^{-1}).
\end{aligned}$$

□

*Proof of Lemma* 4. From the Cauchy-Schwarz inequality, we have

$$0 < \frac{\tau_{1,1}^2}{N_1 \tau_{1,2}} \leq 1,$$

and so

$$\lim_{N_1 \to \infty} \frac{\tau_{1,1}^2}{N_1 \tau_{1,2}} = c \in [0, 1).$$

In addition, it holds that

$$\frac{(N_1 - k_1)^2}{N_1} \leq \tau_{1,1} \leq N_1 - k_1,$$

and so

$$\frac{\tau_{1,1}}{N_1} \asymp 1,$$

where the notation $\asymp$ is defined as follows.

$$A \asymp B \overset{\text{def}}{\Longleftrightarrow} \frac{A}{B} = O(1) \quad \text{and} \quad \frac{B}{A} = O(1).$$

Then we find that

$$\nu_1 = \frac{\dfrac{(N_1-k_1)^2}{(N_1-k_1-1)(N_1-k_1+2)} - \dfrac{N_1}{(N_1-k_1-1)(N_1-k_1+2)}\dfrac{\tau_{1,1}^2}{N_1\tau_{1,2}}}{1-\dfrac{3N_1}{(N_1-k_1)(N_1-k_1+2)}\dfrac{\tau_{1,1}^2}{N_1\tau_{1,2}}} \to 1 \quad (N_1\to\infty),$$

$$N_1^2\nu_2 = \frac{\dfrac{N_1^2}{(N_1-k_1-1)(N_1-k_1+2)}\left\{(N_1-k_1)-\dfrac{\tau_{1,1}^2}{\tau_{1,2}}\right\}}{1-\dfrac{3N_1}{(N_1-k_1)(N_1-k_1+2)}\dfrac{\tau_{1,1}^2}{N_1\tau_{1,2}}} \to c_1\in\mathbb{R} \quad (N_1\to\infty),$$

$$N_1\nu_3 = \frac{\dfrac{N_1}{N_1-k_1+2}\dfrac{N_1}{\tau_{1,1}}\dfrac{\tau_{1,1}^2}{N_1\tau_{1,2}}}{1-\dfrac{3N_1}{(N_1-k_1)(N_1-k_1+2)}\dfrac{\tau_{1,1}^2}{N_1\tau_{1,2}}} \to c_2\in\mathbb{R} \quad (N_1\to\infty),$$

where we use Lemma 10 for the second convergence. It also follows from Lemma 10 that

$$\begin{aligned}
N_1\{\nu_1-(N_1-k_1)\nu_3\} &= N_1\frac{(N_1-k_1)^2(\tau_{1,2}-\tau_{1,1})-\tau_{1,1}^2+(N_1-k_1)\tau_{1,1}}{\dfrac{N_1-k_1-1}{N_1-k_1}\{(N_1-k_1)(N_1-k_1+2)\tau_{1,2}-3\tau_{1,1}^2\}}\\
&= \left\{1-\frac{3N_1}{(N_1-k_1+2)(N_1-k_1)}\frac{\tau_{1,1}^2}{N_1\tau_{1,2}}\right\}^{-1}\left[\frac{(N_1-k_1)^2}{(N_1-k_1-1)(N_1-k_1+2)}\right.\\
&\quad\cdot\left\{N_1\left(1-\frac{\tau_{1,1}}{\tau_{1,2}}\right)\right\} - \frac{N_1^2}{(N_1-k_1-1)(N_1-k_1+2)}\frac{\tau_{1,1}^2}{N_1\tau_{1,2}}\\
&\quad\left.+\frac{N_1(N_1-k_1)}{(N_1-k_1-1)(N_1-k_1+2)}\frac{N_1}{\tau_{1,1}}\frac{\tau_{1,1}^2}{N_1\tau_{1,2}}\right]\\
&\to c_4\in\mathbb{R} \quad (N_1\to\infty).
\end{aligned}$$

□

*S3.2. Proof of Lemma* 5

In this section, we give a proof for Lemma 5. In this proof, the following lemmas (Lemma 11-12) are used.

**Lemma 11.** *For square matrices* $\boldsymbol{A}$ *and* $\boldsymbol{B}$,

(i) $\operatorname{tr}((\boldsymbol{A}+\boldsymbol{B})\odot(\boldsymbol{A}+\boldsymbol{B})) \le 2\{\operatorname{tr}(\boldsymbol{A}\odot\boldsymbol{A})+\operatorname{tr}(\boldsymbol{B}\odot\boldsymbol{B})\}$,

(ii) $|\operatorname{tr}((\boldsymbol{A}+\boldsymbol{B})\odot(\boldsymbol{A}+\boldsymbol{B}))-\operatorname{tr}(\boldsymbol{A}\odot\boldsymbol{A})| \le 2\sqrt{\operatorname{tr}(\boldsymbol{A}\odot\boldsymbol{A})\operatorname{tr}(\boldsymbol{B}\odot\boldsymbol{B})}+\operatorname{tr}(\boldsymbol{B}\odot\boldsymbol{B})$.

**Lemma 12.** *For* $\boldsymbol{Z} = (\boldsymbol{z}_1, \dots, \boldsymbol{z}_{N_1})'$,

$$\text{(i)} \quad E[\operatorname{tr}(\odot^2(\boldsymbol{Z}\boldsymbol{\Upsilon}_1'\boldsymbol{\Upsilon}_1\boldsymbol{Z}'\boldsymbol{\Pi}_{\boldsymbol{A}_1}))] \le \{\mathfrak{q} + \operatorname{tr}(\boldsymbol{\Psi}_1^2)\}\operatorname{tr}(\boldsymbol{\Pi}_{\boldsymbol{A}_1}),$$

$$\text{(ii)} \quad E[\operatorname{tr}(\odot^2(\boldsymbol{\Pi}_{\boldsymbol{A}_1}\boldsymbol{Z}\boldsymbol{\Upsilon}_1'\boldsymbol{\Upsilon}_1\boldsymbol{Z}'\boldsymbol{\Pi}_{\boldsymbol{A}_1}))] \le \{2\mathfrak{q} + 6\operatorname{tr}(\boldsymbol{\Psi}_1^2) + 3(\operatorname{tr}(\boldsymbol{\Psi}_1))^2\}\operatorname{tr}(\boldsymbol{\Pi}_{\boldsymbol{A}_1}).$$

*Proof of Lemma* 11. For $\boldsymbol{A} = (a_{ij}) : N \times N$ and $\boldsymbol{B} = (b_{ij}) : N \times N$,

$$\operatorname{tr}((\boldsymbol{A}+\boldsymbol{B}) \odot (\boldsymbol{A}+\boldsymbol{B})) = \sum_{i=1}^{N}(a_{ii}+b_{ii})^2 \le 2\sum_{i=1}^{N}(a_{ii}^2 + b_{ii}^2) = 2\{\operatorname{tr}(\boldsymbol{A}\odot\boldsymbol{A}) + \operatorname{tr}(\boldsymbol{B}\odot\boldsymbol{B})\},$$

where the inequality follows from the Cauchy-Schwarz inequality. In addition,

$$\begin{aligned}
&|\operatorname{tr}((\boldsymbol{A}+\boldsymbol{B}) \odot (\boldsymbol{A}+\boldsymbol{B})) - \operatorname{tr}(\boldsymbol{A}\odot\boldsymbol{A})| = \left|\sum_{i=1}^{N}(a_{ii}+b_{ii})^2 - \sum_{i=1}^{N} a_{ii}^2\right| \\
&= \left|2\sum_{i=1}^{N} a_{ii}b_{ii} + \sum_{i=1}^{N} b_{ii}^2\right| \le 2\left|\sum_{i=1}^{N} a_{ii}b_{ii}\right| + \sum_{i=1}^{N} b_{ii}^2 \le 2\sqrt{\sum_{i=1}^{N} a_{ii}^2 \sum_{i=1}^{N} b_{ii}^2} + \sum_{i=1}^{N} b_{ii}^2 \\
&= 2\sqrt{\operatorname{tr}(\boldsymbol{A}\odot\boldsymbol{A})\operatorname{tr}(\boldsymbol{B}\odot\boldsymbol{B})} + \operatorname{tr}(\boldsymbol{B}\odot\boldsymbol{B}),
\end{aligned}$$

where the last inequality follows from the Cauchy-Schwarz inequality. □

*Proof of Lemma* 12. It can be described that

$$\begin{aligned}
&\operatorname{tr}(\odot^2(\boldsymbol{Z}\boldsymbol{\Upsilon}_1'\boldsymbol{\Upsilon}_1\boldsymbol{Z}'\boldsymbol{\Pi}_{\boldsymbol{A}_1})) \\
&= \sum_{i=1}^{N_1}\Bigg[(\boldsymbol{z}_i'\boldsymbol{\Upsilon}_1'\boldsymbol{\Upsilon}_1\boldsymbol{z}_i)^2 p_{ii}^2 + 2\boldsymbol{z}_i'\boldsymbol{\Upsilon}_1'\boldsymbol{\Upsilon}_1\boldsymbol{z}_i p_{ii}\sum_{\substack{k=1\\k\ne i}}^{N_1}\boldsymbol{z}_i'\boldsymbol{\Upsilon}_1'\boldsymbol{\Upsilon}_1\boldsymbol{z}_k p_{ki} \\
&\quad + \sum_{\substack{k=1\\k\ne i}}^{N_1}(\boldsymbol{z}_i'\boldsymbol{\Upsilon}_1'\boldsymbol{\Upsilon}_1\boldsymbol{z}_k p_{ki})^2 + \sum_{\substack{k=1\\k\ne i}}^{N_1}\sum_{\substack{\ell=1\\\ell\ne k,i}}^{N_1}\boldsymbol{z}_i'\boldsymbol{\Upsilon}_1'\boldsymbol{\Upsilon}_1\boldsymbol{z}_k\boldsymbol{z}_i'\ \boldsymbol{\Upsilon}_1'\boldsymbol{\Upsilon}_1\boldsymbol{z}_\ell p_{ki}p_{\ell i}\Bigg], \\
&\operatorname{tr}(\odot^2(\boldsymbol{\Pi}_{\boldsymbol{A}_1}\boldsymbol{Z}\boldsymbol{\Upsilon}_1'\boldsymbol{\Upsilon}_1\boldsymbol{Z}'\boldsymbol{\Pi}_{\boldsymbol{A}_1})) \\
&= \sum_{i=1}^{N_1}\Bigg[p_{ii}^2\boldsymbol{z}_i'\boldsymbol{\Upsilon}_1'\boldsymbol{\Upsilon}_1\boldsymbol{z}_i + \sum_{\substack{k=1\\k\ne i}}^{N_1}p_{ik}^2\boldsymbol{z}_k\boldsymbol{\Upsilon}_1'\boldsymbol{\Upsilon}_1\boldsymbol{z}_k + 2\sum_{\substack{k=1\\k\ne i}}^{N_1}p_{ii}p_{ik}\boldsymbol{z}_k'\boldsymbol{\Upsilon}_1'\boldsymbol{\Upsilon}_1\boldsymbol{z}_i \\
&\quad + \sum_{\substack{k=1\\k\ne i}}^{N_1}\sum_{\substack{\ell=1\\\ell\ne i,k}}^{N_1}p_{i\ell}p_{ik}\boldsymbol{z}_k'\boldsymbol{\Upsilon}_1'\boldsymbol{\Upsilon}_1\boldsymbol{z}_\ell\Bigg]^2,
\end{aligned}$$

and so

$$E\left[\operatorname{tr}(\odot^2(\boldsymbol{Z}\boldsymbol{\Upsilon}_1'\boldsymbol{\Upsilon}_1\boldsymbol{Z}'\boldsymbol{\Pi}_{\boldsymbol{A}_1}))\right] = E\left[(\boldsymbol{z}_1'\boldsymbol{\Upsilon}_1'\boldsymbol{\Upsilon}_1\boldsymbol{z}_1)^2\right]\sum_{i=1}^{N_1} p_{ii}^2 + \operatorname{tr}(\boldsymbol{\Psi}_1^2)\sum_{i,j}^{N_1} p_{ij}^2,$$

$$\begin{aligned} E\left[\operatorname{tr}(\odot^2(\boldsymbol{\Pi}_{\boldsymbol{A}_1}\boldsymbol{Z}\boldsymbol{\Upsilon}_1'\boldsymbol{\Upsilon}_1\boldsymbol{Z}'\boldsymbol{\Pi}_{\boldsymbol{A}_1}))\right] = \sum_{i=1}^{N_1}\Bigg[ & p_{ii}^4 E\left[(\boldsymbol{z}_1'\boldsymbol{\Upsilon}_1'\boldsymbol{\Upsilon}_1\boldsymbol{z}_1)^2\right] + \sum_{\substack{k=1\\k\neq i}}^{N_1} p_{ik}^4 E\left[(\boldsymbol{z}_1'\boldsymbol{\Upsilon}_1'\boldsymbol{\Upsilon}_1\boldsymbol{z}_1)^2\right] \\ & + \sum_{\substack{k=1\\k\neq i}}^{N_1}\sum_{\substack{\ell=1\\ \ell\neq i,k}}^{N_1} p_{ik}^2 p_{i\ell}^2 (\operatorname{tr}(\boldsymbol{\Psi}_1))^2 + 4\sum_{\substack{k=1\\k\neq i}}^{N_1} p_{ii}^2 p_{ik}^2 \operatorname{tr}(\boldsymbol{\Psi}_1^2) \\ & + 2\sum_{\substack{k=1\\k\neq i}}^{N_1}\sum_{\substack{\ell=1\\ \ell\neq i,k}}^{N_1} p_{ik}^2 p_{\ell i}^2 \operatorname{tr}(\boldsymbol{\Psi}_1^2) + 2p_{ii}^2 \sum_{\substack{k=1\\k\neq i}}^{N_1} p_{ik}^2 (\operatorname{tr}(\boldsymbol{\Psi}_1))^2 \Bigg]. \end{aligned}$$

The assertions are followed from (13), (14) and the following inequalities:

$$0 \le \sum_{i,j}^{N_1} p_{ii}^2 p_{ij}^2 \le \sum_{i,j}^{N_1} p_{ij}^2 \le \operatorname{tr}(\boldsymbol{\Pi}_{\boldsymbol{A}_1}^2) \le \operatorname{tr}(\boldsymbol{\Pi}_{\boldsymbol{A}_1}),$$

$$0 \le \sum_{i,j,k}^{N_1} p_{ij}^2 p_{ik}^2 \le \sum_{i=1}^{N_1}\left(\sum_{j=1}^{N_1} p_{ij}^2\right)\left(\sum_{k=1}^{N_1} p_{ik}^2\right) = \sum_{i=1}^{N_1} p_{ii}^2 \le \operatorname{tr}(\boldsymbol{\Pi}_{\boldsymbol{A}_1}).$$

□

*Proof of Lemma* 5 (i). It holds that $E[\operatorname{tr}(\boldsymbol{S}_1)/\operatorname{tr}(\boldsymbol{\Psi}_1)] = 1$ and

$$\operatorname{Var}\left(\frac{\operatorname{tr}(\boldsymbol{S}_1)}{\operatorname{tr}(\boldsymbol{\Psi}_1)}\right) = \frac{\tau_{1,1}}{(N_1-k_1)^2}\frac{\mathfrak{q} - 2\operatorname{tr}(\boldsymbol{\Psi}_1^2) - (\operatorname{tr}(\boldsymbol{\Psi}_1))^2}{(\operatorname{tr}(\boldsymbol{\Psi}_1))^2} + \frac{2}{N_1-k}\frac{\operatorname{tr}(\boldsymbol{\Psi}_1^2)}{(\operatorname{tr}(\boldsymbol{\Psi}_1))^2};$$

and thus established that $\operatorname{Var}(\operatorname{tr}(\boldsymbol{S}_1)/\operatorname{tr}(\boldsymbol{\Psi}_1)) \to 0$ as $\min\{N_1, p\} \to \infty$. Consequently, the assertion (i) holds from the Chebyshev's inequality. □

*Proof of Lemma* 5 (ii). It can be described that

$$\operatorname{tr}(\boldsymbol{S}_1^2) = \frac{1}{(N_1-k_1)^2}\left\{\operatorname{tr}((\boldsymbol{Z}\boldsymbol{\Upsilon}_1'\boldsymbol{\Upsilon}_1\boldsymbol{Z}')^2) - 2\operatorname{tr}(\boldsymbol{\Pi}_{\boldsymbol{A}_1}(\boldsymbol{Z}\boldsymbol{\Upsilon}_1'\boldsymbol{\Upsilon}_1\boldsymbol{Z}')^2) + \operatorname{tr}((\boldsymbol{\Pi}_{\boldsymbol{A}_1}\boldsymbol{Z}\boldsymbol{\Upsilon}_1'\boldsymbol{\Upsilon}_1\boldsymbol{Z}')^2)\right\}.$$

Using this expression, we have

$$\begin{aligned} & \left|\frac{\operatorname{tr}(\boldsymbol{S}_1^2)}{\operatorname{tr}(\boldsymbol{\Psi}_1^2)} - \frac{1}{(N_1-k_1)^2}\frac{\operatorname{tr}((\boldsymbol{Z}\boldsymbol{\Upsilon}_1'\boldsymbol{\Upsilon}_1\boldsymbol{Z}')^2)}{\operatorname{tr}(\boldsymbol{\Psi}_1^2)}\right| \\ & \le \frac{1}{(N_1-k_1)^2}\left\{\frac{2\operatorname{tr}(\boldsymbol{\Pi}_{\boldsymbol{A}_1}(\boldsymbol{Z}\boldsymbol{\Upsilon}_1'\boldsymbol{\Upsilon}_1\boldsymbol{Z}')^2)}{\operatorname{tr}(\boldsymbol{\Psi}_1^2)} + \frac{|\operatorname{tr}((\boldsymbol{\Pi}_{\boldsymbol{A}_1}\boldsymbol{Z}\boldsymbol{\Upsilon}_1'\boldsymbol{\Upsilon}_1\boldsymbol{Z}')^2)|}{\operatorname{tr}(\boldsymbol{\Psi}_1^2)}\right\}. \end{aligned}$$

From the Markov inequality, $\forall\delta>0$,

$$
\begin{aligned}
&P\left(\left|\frac{\operatorname{tr}(\boldsymbol{S}_1^2)}{\operatorname{tr}(\boldsymbol{\Psi}_1^2)}-\frac{1}{(N_1-k_1)^2}\frac{\operatorname{tr}((\boldsymbol{Z}\boldsymbol{\Upsilon}_1'\boldsymbol{\Upsilon}_1\boldsymbol{Z}')^2)}{\operatorname{tr}(\boldsymbol{\Psi}_1^2)}\right|>\delta\right)\\
&<\frac{2E[\operatorname{tr}(\boldsymbol{\Pi}_{\boldsymbol{A}_1}(\boldsymbol{Z}\boldsymbol{\Upsilon}_1'\boldsymbol{\Upsilon}_1\boldsymbol{Z}')^2)]+E[|\operatorname{tr}((\boldsymbol{\Pi}_{\boldsymbol{A}_1}\boldsymbol{Z}\boldsymbol{\Upsilon}_1'\boldsymbol{\Upsilon}_1\boldsymbol{Z}')^2)|]}{\delta(N_1-k_1)^2\operatorname{tr}(\boldsymbol{\Psi}_1^2)}\\
&\leq\frac{(2+\sqrt{k_1})E[\operatorname{tr}(\boldsymbol{\Pi}_{\boldsymbol{A}_1}(\boldsymbol{Z}\boldsymbol{\Upsilon}_1'\boldsymbol{\Upsilon}_1\boldsymbol{Z}')^2)]}{\delta(N_1-k_1)^2\operatorname{tr}(\boldsymbol{\Psi}_1^2)},
\end{aligned}
$$

where the last inequality follows from Cauchy-Schwarz inequality:

$$
\begin{aligned}
&|\operatorname{tr}(\boldsymbol{\Pi}_{\boldsymbol{A}_1}\boldsymbol{Z}\boldsymbol{\Upsilon}_1'\boldsymbol{\Upsilon}_1\boldsymbol{Z}')^2)|\\
&\leq\sqrt{\operatorname{tr}(\boldsymbol{\Pi}_{\boldsymbol{A}_1}^2)}\sqrt{\operatorname{tr}((\boldsymbol{Z}\boldsymbol{\Upsilon}_1'\boldsymbol{\Upsilon}_1\boldsymbol{Z}'\boldsymbol{\Pi}_{\boldsymbol{A}_1}\boldsymbol{Z}\boldsymbol{\Upsilon}_1'\boldsymbol{\Upsilon}_1\boldsymbol{Z}')^2)}\\
&\leq\sqrt{k_1}\operatorname{tr}(\boldsymbol{Z}\boldsymbol{\Upsilon}_1'\boldsymbol{\Upsilon}_1\boldsymbol{Z}'\boldsymbol{\Pi}_{\boldsymbol{A}_1}\boldsymbol{Z}\boldsymbol{\Upsilon}_1'\boldsymbol{\Upsilon}_1\boldsymbol{Z}').
\end{aligned}
$$

Letting $(i,j)$-th elements of the matrix $(\boldsymbol{Z}\boldsymbol{\Upsilon}_1'\boldsymbol{\Upsilon}_1\boldsymbol{Z}')^2$ be $(\boldsymbol{Z}\boldsymbol{\Upsilon}_1'\boldsymbol{\Upsilon}_1\boldsymbol{Z}')^2_{ij}$, it can be described that

$$
E[(\boldsymbol{Z}\boldsymbol{\Upsilon}_1'\boldsymbol{\Upsilon}_1\boldsymbol{Z}')^2_{ij}]=\begin{cases}\mathfrak{q}+(N_1-1)\operatorname{tr}(\boldsymbol{\Psi}_1^2), & i=j,\\ 0 & i\neq j.\end{cases}
$$

The assertion (ii) holds since

$$
\begin{aligned}
E\left[\frac{\operatorname{tr}(\boldsymbol{\Pi}_{\boldsymbol{A}_1}(\boldsymbol{Z}\boldsymbol{\Upsilon}_1'\boldsymbol{\Upsilon}_1\boldsymbol{Z}')^2)}{(N_1-k_1)^2\operatorname{tr}(\boldsymbol{\Psi}_1^2)}\right]&=\frac{\mathfrak{q}+(N_1-1)\operatorname{tr}(\boldsymbol{\Psi}_1^2)}{(\operatorname{tr}(\boldsymbol{\Psi}_1))^2}\frac{(\operatorname{tr}(\boldsymbol{\Psi}_1))^2}{p\operatorname{tr}(\boldsymbol{\Psi}_1^2)}\frac{p\operatorname{tr}(\boldsymbol{\Pi}_{\boldsymbol{A}_1})}{(N_1-k_1)^2}\\
&\leq\left|\frac{\mathfrak{q}}{(\operatorname{tr}(\boldsymbol{\Psi}_1))^2}\right|\frac{(\operatorname{tr}(\boldsymbol{\Psi}_1))^2}{p\operatorname{tr}(\boldsymbol{\Psi}_1^2)}\frac{pk_1}{(N_1-k_1)^2}+\frac{k_1(N_1-1)}{(N_1-k_1)^2}\\
&\to 0\quad(\min\{N_1,p\}\to\infty\text{ and }p/N_1\to c_1\in(0,\infty)).
\end{aligned}
$$

□

*Proof of Lemma* 5 (iii). It can be described that

$$
Q_1=\frac{\operatorname{tr}\left(\odot^2\left\{(\boldsymbol{I}_N-\boldsymbol{\Pi}_{\boldsymbol{A}_1})\boldsymbol{Z}\boldsymbol{\Upsilon}_1'\boldsymbol{\Upsilon}_1\boldsymbol{Z}'(\boldsymbol{I}_N-\boldsymbol{\Pi}_{\boldsymbol{A}_1})\right\}\right)}{N_1-k_1}.
$$

Write

$$
\frac{Q_1}{p\operatorname{tr}(\boldsymbol{\Psi}_1^2)}=\operatorname{tr}(\odot^2(\boldsymbol{W}_1+\boldsymbol{W}_2+\boldsymbol{W}_3+\boldsymbol{W}_4)),
$$

where

$$\boldsymbol{W}_1 = \frac{\boldsymbol{Z}\boldsymbol{\Upsilon}_1'\boldsymbol{\Upsilon}_1\boldsymbol{Z}'}{\sqrt{(N_1-k_1)p\operatorname{tr}(\boldsymbol{\Psi}_1^2)}}, \boldsymbol{W}_2 = -\frac{\boldsymbol{Z}\boldsymbol{\Upsilon}_1'\boldsymbol{\Upsilon}_1\boldsymbol{Z}'\boldsymbol{\Pi}_{\boldsymbol{A}_1}}{\sqrt{(N_1-k_1)p\operatorname{tr}(\boldsymbol{\Psi}_1^2)}},$$
$$\boldsymbol{W}_3 = -\frac{\boldsymbol{\Pi}_{\boldsymbol{A}_1}\boldsymbol{Z}\boldsymbol{\Upsilon}_1'\boldsymbol{\Upsilon}_1\boldsymbol{Z}'}{\sqrt{(N_1-k_1)p\operatorname{tr}(\boldsymbol{\Psi}_1^2)}}, \boldsymbol{W}_4 = \frac{\boldsymbol{\Pi}_{\boldsymbol{A}_1}\boldsymbol{Z}\boldsymbol{\Upsilon}_1'\boldsymbol{\Upsilon}_1\boldsymbol{Z}'\boldsymbol{\Pi}_{\boldsymbol{A}_1}}{\sqrt{(N_1-k_1)p\operatorname{tr}(\boldsymbol{\Psi}_1^2)}}.$$

From Lemma 11, we have

$$\begin{aligned}
&\left|\operatorname{tr}(\odot^2(\boldsymbol{W}_1+\boldsymbol{W}_2+\boldsymbol{W}_3+\boldsymbol{W}_4)) - \operatorname{tr}(\odot^2\boldsymbol{W}_1)\right| \\
&\le 2\sqrt{\operatorname{tr}(\odot^2\boldsymbol{W}_1)\operatorname{tr}(\odot^2(\boldsymbol{W}_2+\boldsymbol{W}_3+\boldsymbol{W}_4))} + \operatorname{tr}(\odot^2(\boldsymbol{W}_2+\boldsymbol{W}_3+\boldsymbol{W}_4)) \\
&\le 2\sqrt{\operatorname{tr}(\odot^2\boldsymbol{W}_1)\cdot 2\left[\operatorname{tr}(\odot^2(\boldsymbol{W}_2+\boldsymbol{W}_3)) + \operatorname{tr}(\odot^2\boldsymbol{W}_4)\right]} + 2\left[\operatorname{tr}(\odot^2(\boldsymbol{W}_2+\boldsymbol{W}_3)) + \operatorname{tr}(\odot^2\boldsymbol{W}_4)\right] \\
&\le 2\sqrt{\operatorname{tr}(\odot^2\boldsymbol{W}_1)\cdot 2\left[2\{\operatorname{tr}(\odot^2\boldsymbol{W}_2) + \operatorname{tr}(\odot^2\boldsymbol{W}_3)\} + \operatorname{tr}(\odot^2\boldsymbol{W}_4)\right]} \\
&\quad + 2\left[2\{\operatorname{tr}(\odot^2\boldsymbol{W}_2) + \operatorname{tr}(\odot^2\boldsymbol{W}_3)\} + \operatorname{tr}(\odot^2\boldsymbol{W}_4)\right] \\
&= 2\sqrt{\operatorname{tr}(\odot^2\boldsymbol{W}_1)(4\operatorname{tr}(\odot^2\boldsymbol{W}_2) + 4\operatorname{tr}(\odot^2\boldsymbol{W}_3) + 2\operatorname{tr}(\odot^2\boldsymbol{W}_4))} \\
&\quad + 4\operatorname{tr}(\odot^2\boldsymbol{W}_2) + 4\operatorname{tr}(\odot^2\boldsymbol{W}_3) + 2\operatorname{tr}(\odot^2\boldsymbol{W}_4). \qquad (15)
\end{aligned}$$

From the Markov inequality, $\forall\delta > 0$,

$$\begin{aligned}
&P\left(\left|\frac{Q_1}{p\operatorname{tr}(\boldsymbol{\Psi}_1^2)} - \frac{1}{N_1-k_1}\frac{\operatorname{tr}((\boldsymbol{Z}\boldsymbol{\Upsilon}_1'\boldsymbol{\Upsilon}_1\boldsymbol{Z})\odot(\boldsymbol{Z}\boldsymbol{\Upsilon}_1'\boldsymbol{\Upsilon}_1\boldsymbol{Z}))}{p\operatorname{tr}(\boldsymbol{\Psi}_1^2)}\right| > \delta\right) \\
&\le \delta^{-1}(2\sqrt{E[\operatorname{tr}(\odot^2\boldsymbol{W}_1)](E[4\operatorname{tr}(\odot^2\boldsymbol{W}_2) + 4\operatorname{tr}(\odot^2\boldsymbol{W}_3) + 2\operatorname{tr}(\odot^2\boldsymbol{W}_4)])} \\
&\quad + E[4\operatorname{tr}(\odot^2\boldsymbol{W}_2) + 4\operatorname{tr}(\odot^2\boldsymbol{W}_3) + 2\operatorname{tr}(\odot^2\boldsymbol{W}_4)]),
\end{aligned}$$

where the inequality follows from Cauchy-Schwarz inequality for (15). The assertion of the lemma is followed from

$$E[\operatorname{tr}(\odot^2\boldsymbol{W}_1)] = O(1), \quad E[\operatorname{tr}(\odot^2\boldsymbol{W}_2)] = o(1), \quad E[\operatorname{tr}(\odot^2\boldsymbol{W}_3)] = o(1), \quad E[\operatorname{tr}(\odot^2\boldsymbol{W}_4)] = o(1)$$

as $\min\{N_1, p\} \to \infty$, which are found from Lemma 12. □

*S3.3. Proof of Lemma 6*

In this section, we give a proof for Lemma 6.

*Proof of Lemma* 6 (i). From the Markov inequality, $\forall\delta > 0$,

$$P\left(\left|\frac{1}{N_1^2}\sum_{i=1}^{N_1}\frac{(\boldsymbol{z}_i'\boldsymbol{\Upsilon}_1'\boldsymbol{\Upsilon}_1\boldsymbol{z}_i)^2}{(\operatorname{tr}(\boldsymbol{\Psi}_1))^2}\right| > \delta\right) < \delta^{-1}E\left[\frac{1}{N_1^2}\sum_{i=1}^{N_1}\frac{(\boldsymbol{z}_i'\boldsymbol{\Upsilon}_1'\boldsymbol{\Upsilon}_1\boldsymbol{z}_i)^2}{(\operatorname{tr}(\boldsymbol{\Psi}_1))^2}\right] = \frac{\mathfrak{q}}{N_1(\operatorname{tr}(\boldsymbol{\Psi}_1))^2\delta} \to 0$$

as $\min\{N_1, p\} \to \infty$. □

*Proof of Lemma* 6 (ii). In the original paper, we have shown that $E[B_1^2] \to 0$ as $\min\{N, p\} \to \infty$. Modifying the proof, we can show Lemma 6 (ii). $\square$

## S4. Specific results for proposed test

We introduce the specific results obtained for the proposed test (12), all of which are heterogeneous. In this section, we assume A1-A3 and D1-D2.

### *S4.1. Test for one-way MANOVA*

For the generalized multivariate linear model (1), consider the case in which $k = g$, $q = p$, and $\boldsymbol{A}$ is given as in (9):

$$\boldsymbol{\Theta} = (\boldsymbol{\mu}_1, \boldsymbol{\mu}_2, \ldots, \boldsymbol{\mu}_g)', \quad \boldsymbol{B} = \boldsymbol{I}_p. \tag{16}$$

Set $\boldsymbol{R} = \boldsymbol{I}_p$ in the bilateral linear hypothesis (2). Then, the null hypothesis becomes $H_0 : \boldsymbol{L\Theta} = \boldsymbol{O}$. Under this setting,

$$\boldsymbol{\Pi}_{\mathrm{H}} = \begin{pmatrix} \eta_{11}\boldsymbol{\Pi}_{N_1} & \eta_{12}(N_1N_2)^{-1/2}\mathbf{1}_{N_1}\mathbf{1}'_{N_2} & \cdots & \eta_{1g}(N_1N_g)^{-1/2}\mathbf{1}_{N_1}\mathbf{1}'_{N_g} \\ \eta_{21}(N_2N_1)^{-1/2}\mathbf{1}_{N_2}\mathbf{1}'_{N_1} & \eta_{22}\boldsymbol{\Pi}_{N_2} & \cdots & \eta_{2g}(N_2N_g)^{-1/2}\mathbf{1}_{N_2}\mathbf{1}'_{N_g} \\ \vdots & \vdots & \ddots & \vdots \\ \eta_{g1}(N_gN_1)^{-1/2}\mathbf{1}_{N_g}\mathbf{1}'_{N_1} & \eta_{g2}(N_2N_2)^{-1/2}\mathbf{1}_{N_g}\mathbf{1}'_{N_2} & \cdots & \eta_{gg}\boldsymbol{\Pi}_{N_g} \end{pmatrix},$$

where

$$\eta_{ij} = \frac{1}{\sqrt{N_iN_j}}\boldsymbol{\ell}'_i\left(\boldsymbol{L}\,\mathrm{diag}(1/N_1, \ldots, 1/N_g)\boldsymbol{L}'\right)^{-1}\boldsymbol{\ell}_j, \quad i, j \in [\![g]\!], \quad \boldsymbol{L} = (\boldsymbol{\ell}_1, \boldsymbol{\ell}_2, \ldots, \boldsymbol{\ell}_g),$$

$$\boldsymbol{\Pi}_{\boldsymbol{A}} = \mathrm{diag}(\boldsymbol{\Pi}_{N_1}, \boldsymbol{\Pi}_{N_2}, \ldots, \boldsymbol{\Pi}_{N_g}), \quad \boldsymbol{\Pi}_{N_i} = \frac{1}{N_i}\mathbf{1}_{N_i}\mathbf{1}'_{N_i}, \quad i \in [\![g]\!].$$

Because

$$\begin{aligned} &(\boldsymbol{I}_N - \boldsymbol{\Pi}_{\boldsymbol{A}}) \odot (\boldsymbol{I}_N - \boldsymbol{\Pi}_{\boldsymbol{A}}) \\ &= (\boldsymbol{I}_N - \mathrm{diag}(\boldsymbol{\Pi}_{N_1}, \boldsymbol{\Pi}_{N_2}, \ldots, \boldsymbol{\Pi}_{N_g})) \odot (\boldsymbol{I}_N - \mathrm{diag}(\boldsymbol{\Pi}_{N_1}, \boldsymbol{\Pi}_{N_2}, \ldots, \boldsymbol{\Pi}_{N_g})) \end{aligned}$$

is non-singular, the inverse matrix exists, which can be described as follows:

$$\{(\boldsymbol{I}_N - \boldsymbol{\Pi}_{\boldsymbol{A}}) \odot (\boldsymbol{I}_N - \boldsymbol{\Pi}_{\boldsymbol{A}})\}^{-1} = \mathrm{diag}(\boldsymbol{M}_1, \ldots, \boldsymbol{M}_g),$$

where

$$\boldsymbol{M}_i = \frac{N_i}{N_i - 2}\left(\boldsymbol{I}_{N_i} - \frac{1}{N_i - 1}\boldsymbol{\Pi}_{N_i}\right), \quad i \in [\![g]\!].$$

Then, the linear equation (5) has the following unique solution:

$$(d_1, d_2, \ldots, d_N)' = \left(\eta_{11}(N_1 - 1)^{-1}\mathbf{1}'_{N_1}, \eta_{22}(N_2 - 1)^{-1}\mathbf{1}'_{N_2}, \ldots, \eta_{gg}(N_g - 1)^{-1}\mathbf{1}'_{N_g}\right)'.$$

After simple calculations, we can obtain the following:

$$\begin{aligned}\boldsymbol{\Omega} &= \boldsymbol{\Pi}_{\mathrm{H}} - (\boldsymbol{I}_N - \boldsymbol{\Pi}_{\mathrm{A}})\boldsymbol{D}(\boldsymbol{I}_N - \boldsymbol{\Pi}_{\mathrm{A}}) \\ &= \begin{pmatrix} \frac{\eta_{11}}{N_1-1}(N_1\boldsymbol{\Pi}_{N_1} - \boldsymbol{I}_{N_1}) & \frac{\eta_{12}}{\sqrt{N_1N_2}}\boldsymbol{1}_{N_1}\boldsymbol{1}_{N_2}' & \cdots & \frac{\eta_{1g}}{\sqrt{N_1N_g}}\boldsymbol{1}_{N_1}\boldsymbol{1}_{N_g}' \\ \frac{\eta_{21}}{\sqrt{N_2N_1}}\boldsymbol{1}_{N_2}\boldsymbol{1}_{N_1}' & \frac{\eta_{22}}{N_2-1}(N_2\boldsymbol{\Pi}_{N_2} - \boldsymbol{I}_{N_2}) & \cdots & \frac{\eta_{2g}}{\sqrt{N_2N_g}}\boldsymbol{1}_{N_2}\boldsymbol{1}_{N_g}' \\ \vdots & \vdots & \ddots & \vdots \\ \frac{\eta_{g1}}{\sqrt{N_gN_1}}\boldsymbol{1}_{N_g}\boldsymbol{1}_{N_1}' & \frac{\eta_{g2}}{\sqrt{N_gN_2}}\boldsymbol{1}_{N_g}\boldsymbol{1}_{N_2}' & \cdots & \frac{\eta_{gg}}{N_g-1}(N_g\boldsymbol{\Pi}_{N_g} - \boldsymbol{I}_{N_g}) \end{pmatrix}. \end{aligned} \tag{17}$$

Note that $\boldsymbol{\mathcal{P}} = \boldsymbol{I}_p$; thus, the testing statistic is described as $T = \mathrm{tr}(\boldsymbol{X}'\boldsymbol{\Omega}\boldsymbol{X})$. It then follows from (17) that

$$\hat{\sigma}_0^2 = 2\,\mathrm{tr}((\boldsymbol{\Omega} \odot \boldsymbol{\Omega})\hat{\boldsymbol{V}}) = 2\sum_{i=1}^{g} \frac{N_i}{N_i - 1}\eta_{ii}^2 \hat{a}_{i,2} + 2\sum_{i,j}^{g} \eta_{ij}^2 \hat{b}_{ij}. \tag{18}$$

First, we handle the case in which $g = 1$, where the null hypothesis becomes $H_0 : \boldsymbol{\mu}_1 = \boldsymbol{0}$. It can be observed that $\eta_{11} = 1$; thus, $\boldsymbol{\Omega} = (N_1 - 1)^{-1}(N_1\boldsymbol{\Pi}_{N_1} - \boldsymbol{I}_{N_1})$. Then,

$$\begin{aligned} T = \mathrm{tr}(\boldsymbol{X}'\boldsymbol{\Omega}\boldsymbol{X}) &= \frac{1}{N_1 - 1}\,\mathrm{tr}\left(\boldsymbol{X}'\left\{(N_1 - 1)\boldsymbol{\Pi}_{N_1} - (\boldsymbol{I}_{N_1} - \boldsymbol{\Pi}_{N_1})\right\}\boldsymbol{X}\right) \\ &= N_1\bar{\boldsymbol{x}}^{(1)'}\bar{\boldsymbol{x}}^{(1)} - \mathrm{tr}(\boldsymbol{S}_1), \end{aligned}$$

where

$$\boldsymbol{S}_i = \frac{1}{N_i - 1}\sum_{j=1}^{N_i}(\boldsymbol{x}_j^{(i)} - \bar{\boldsymbol{x}}^{(i)})(\boldsymbol{x}_j^{(i)} - \bar{\boldsymbol{x}}^{(i)})', \quad i \in [\![g]\!]. \tag{19}$$

This is a one-sample analog of the testing statistic given by Chen and Qin [2]. The null hypothesis $H_0 : \boldsymbol{\mu}_1 = \boldsymbol{0}$ is rejected with the significance level $\varepsilon$ if

$$\frac{T}{\sqrt{\hat{\sigma}_0^2}} = \frac{\bar{\boldsymbol{x}}^{(1)'}\bar{\boldsymbol{x}}^{(1)} - \mathrm{tr}(\boldsymbol{S}_1)/N_1}{\sqrt{2\hat{a}_{1,2}/\mathrm{P}_{N_1,2}}} > \Phi^{-1}(1 - \varepsilon).$$

Next, we treat the multisample problem. Let

$$\boldsymbol{L} = \begin{pmatrix} 1 & 0 & \cdots & 0 & -1 \\ 0 & 1 & \cdots & 0 & -1 \\ \vdots & \vdots & \ddots & \vdots & \vdots \\ 0 & 0 & \cdots & 1 & -1 \end{pmatrix} = (\boldsymbol{I}_{g-1}, -\boldsymbol{1}_{g-1}). \tag{20}$$

Then, $H_0 : \boldsymbol{\mu}_1 = \boldsymbol{\mu}_2 = \cdots = \boldsymbol{\mu}_g$ is equivalent to $H_0 : \boldsymbol{L}\boldsymbol{\Theta} = \boldsymbol{O}$. It follows from (20) that

$$\eta_{ii} = 1 - N_i/N, \quad i \in [\![g]\!]; \quad \eta_{ij} = -\sqrt{N_iN_j}/N, \quad i, j \in [\![g]\!], \quad i \neq j. \tag{21}$$

Thus,

$$(d_1, d_2, \ldots, d_N)' = \left( \frac{1 - N_1/N}{N_1 - 1} \mathbf{1}'_{N_1}, \frac{1 - N_2/N}{N_2 - 1} \mathbf{1}'_{N_2}, \ldots, \frac{1 - N_g/N}{N_g - 1} \mathbf{1}'_{N_1} \right)'.$$

In this case, the following equalities hold.

$$\begin{aligned} \operatorname{tr}(\boldsymbol{X}'(\boldsymbol{I}_N - \boldsymbol{\Pi}_{\mathrm{A}})\boldsymbol{D}(\boldsymbol{I}_N - \boldsymbol{\Pi}_{\mathrm{A}})\boldsymbol{X}) &= \operatorname{tr}\big(\boldsymbol{D}(\boldsymbol{I}_N - \boldsymbol{\Pi}_{\mathrm{A}})\boldsymbol{X}\boldsymbol{X}'(\boldsymbol{I}_N - \boldsymbol{\Pi}_{\mathrm{A}})\big) \\ &= \sum_{i=1}^{g} \left(1 - \frac{N_i}{N}\right) \operatorname{tr}(\boldsymbol{S}_i), \end{aligned}$$

where $\boldsymbol{S}_i$ is defined as (19). Thus, the statistic $T = \operatorname{tr}(\boldsymbol{X}'\boldsymbol{\Omega}\boldsymbol{X})$ can be expressed as

$$\begin{aligned} &\operatorname{tr}(\boldsymbol{X}'\boldsymbol{\Pi}_{\mathrm{H}}\boldsymbol{X}) - \operatorname{tr}(\boldsymbol{X}'(\boldsymbol{I}_N - \boldsymbol{\Pi}_{\mathrm{A}})\boldsymbol{D}(\boldsymbol{I}_N - \boldsymbol{\Pi}_{\mathrm{A}})\boldsymbol{X}) \\ &= \operatorname{tr}(\boldsymbol{S}_{\mathrm{h}}) - \sum_{i=1}^{g} \left(1 - \frac{N_i}{N}\right) \operatorname{tr}(\boldsymbol{S}_i), \end{aligned}$$

which is identical to the statistic $T_{\mathrm{YH}}$ given by Yamada and Himeno [7], where

$$\boldsymbol{S}_{\mathrm{h}} = \sum_{i=1}^{g} N_i(\bar{\boldsymbol{x}}^{(i)} - \bar{\boldsymbol{x}})(\bar{\boldsymbol{x}}^{(i)} - \bar{\boldsymbol{x}})', \quad \bar{\boldsymbol{x}} = N^{-1} \sum_{i=1}^{g} N_i \bar{\boldsymbol{x}}^{(i)}. \tag{22}$$

Specifically, for the case in which $g = 2$, we find that

$$\begin{aligned} \operatorname{tr}(\boldsymbol{S}_{\mathrm{h}}) &= N_1(\bar{\boldsymbol{x}}^{(1)} - \bar{\boldsymbol{x}})'(\bar{\boldsymbol{x}}^{(1)} - \bar{\boldsymbol{x}}) + N_2(\bar{\boldsymbol{x}}^{(2)} - \bar{\boldsymbol{x}})'(\bar{\boldsymbol{x}}^{(2)} - \bar{\boldsymbol{x}}) \\ &= \frac{N_1 N_2^2}{N^2}(\bar{\boldsymbol{x}}^{(1)} - \bar{\boldsymbol{x}}^{(2)})'(\bar{\boldsymbol{x}}^{(1)} - \bar{\boldsymbol{x}}^{(2)}) + \frac{N_1^2 N_2}{N^2}(\bar{\boldsymbol{x}}^{(2)} - \bar{\boldsymbol{x}}^{(1)})'(\bar{\boldsymbol{x}}^{(2)} - \bar{\boldsymbol{x}}^{(1)}) \\ &= \frac{N_1 N_2}{N}(\bar{\boldsymbol{x}}^{(1)} - \bar{\boldsymbol{x}}^{(2)})'(\bar{\boldsymbol{x}}^{(1)} - \bar{\boldsymbol{x}}^{(2)}), \end{aligned}$$

where the second equality follows from $\bar{\boldsymbol{x}} = (N_1/N)\bar{\boldsymbol{x}}^{(1)} + (N_2/N)\bar{\boldsymbol{x}}^{(2)}$; thus,

$$\begin{aligned} \frac{N}{N_1 N_2} T &= (\bar{\boldsymbol{x}}^{(1)} - \bar{\boldsymbol{x}}^{(2)})'(\bar{\boldsymbol{x}}^{(1)} - \bar{\boldsymbol{x}}^{(2)}) - \frac{1}{N_1} \operatorname{tr}(\boldsymbol{S}_1) - \frac{1}{N_2} \operatorname{tr}(\boldsymbol{S}_2) \\ &= \frac{1}{N_1(N_1 - 1)} \sum_{i,j}^{N_1} \boldsymbol{x}_i^{(1)'} \boldsymbol{x}_j^{(1)} + \frac{1}{N_2(N_2 - 1)} \sum_{i,j}^{N_2} \boldsymbol{x}_i^{(2)'} \boldsymbol{x}_j^{(2)} - \frac{2}{N_1 N_2} \sum_{i=1}^{N_1} \sum_{j=1}^{N_2} \boldsymbol{x}_i^{(1)'} \boldsymbol{x}_j^{(2)}, \end{aligned}$$

which is identical to the testing statistic given by Chen and Qin [2]. From the definition of $\boldsymbol{\Omega}$ in (17) and that of $\eta_{ij}$ in (21), the following expression can be obtained:

$$\hat{\sigma}_0^2 = 2\operatorname{tr}((\boldsymbol{\Omega} \odot \boldsymbol{\Omega})\boldsymbol{V}) = 2\sum_{i=1}^{g} \left(1 - \frac{N_i}{N}\right) \frac{N_i}{N_i - 1} \hat{a}_{i,2} + 2\sum_{i,j}^{g} \frac{N_i N_j}{N^2} \hat{b}_{ij} = \hat{\sigma}_{\mathrm{YH}}^2,$$

where $\hat{a}_{i,2}$ is given by (10) and $\hat{b}_{ij} = \operatorname{tr}(\boldsymbol{S}_i \boldsymbol{S}_j)$, $i, j \in [\![g]\!]$, $i \neq j$. Yamada and Himeno [7] used $\hat{\sigma}_{\mathrm{YH}}^2$ as the estimator of $\operatorname{Var}(T_{\mathrm{YH}})$ and showed the asymptotic normality of $T_{\mathrm{YH}}/\sqrt{\hat{\sigma}_{\mathrm{YH}}^2}$. Consequently, the

null hypothesis $H_0 : \boldsymbol{\mu}_1 = \boldsymbol{\mu}_2 = \cdots = \boldsymbol{\mu}_g$ is rejected with the significance level $\varepsilon$ if

$$\frac{T_{\mathrm{YH}}}{\sqrt{\hat{\sigma}^2_{\mathrm{YH}}}} \equiv \frac{T}{\sqrt{\hat{\sigma}^2_0}} > \Phi^{-1}(1-\varepsilon).$$

*S4.2. Test for multivariate linear hypothesis*

We treat the same model as that in Section S4.1, and consider the problem of testing the null hypothesis $H_0 : \boldsymbol{L\Theta} = \boldsymbol{O}$ with $\boldsymbol{\Theta}$ defined as in (16). Zhou et al. [8] proposed testing the statistic $T_{\mathrm{ZGZ}}$, which is defined as follows:

$$T_{\mathrm{ZGZ}} = \sum_{i=1}^{g} c_{ii} S_{ii} + \sum_{i,j}^{g} c_{ij} S_{ij},$$

where

$$\begin{aligned} S_{ii} &= \bar{\boldsymbol{x}}^{(i)\prime}\bar{\boldsymbol{x}}^{(i)} - \frac{\operatorname{tr}\boldsymbol{S}_i}{N_i}, \quad i \in [\![g]\!]; \\ S_{ij} &= \bar{\boldsymbol{x}}^{(i)\prime}\bar{\boldsymbol{x}}^{(j)}, \quad i, j \in [\![g]\!], \quad i \neq j; \\ (c_{ij}) &= \boldsymbol{C} = \boldsymbol{L}'(\boldsymbol{L}\mathrm{diag}(N/N_1, \ldots, N/N_g)\boldsymbol{L}')^{-1}\boldsymbol{L}. \end{aligned}$$

They described that

$$\sigma^2_{\mathrm{ZGZ}} = \mathrm{Var}(T_{\mathrm{ZGZ}}) = 2\left(\sum_{i=1}^{g} \frac{c_{ii}^2 a_{i,2}}{N_i(N_i-1)} + \sum_{i,j}^{g} \frac{c_{ij}^2 b_{ij}}{N_i N_j}\right),$$

and gave its unbiased estimator as follows:

$$\hat{\sigma}^2_{\mathrm{ZGZ}} = 2\left(\sum_{i=1}^{g} \frac{c_{ii}^2 \hat{a}_{i,2}}{N_i(N_i-1)} + \sum_{i,j}^{g} \frac{c_{ij}^2 \hat{b}_{ij}}{N_i N_j}\right).$$

They also showed the asymptotic normality of $T_{\mathrm{ZGZ}}/\sqrt{\hat{\sigma}^2_{\mathrm{ZGZ}}}$, and proposed the following testing criterion with the significance level $\varepsilon$:

$$\frac{T_{\mathrm{ZGZ}}}{\sqrt{\hat{\sigma}^2_{\mathrm{ZGZ}}}} > \Phi^{-1}(1-\varepsilon) \quad \Longrightarrow \quad \text{Reject the null hypothesis } H_0 : \boldsymbol{L\Theta} = \boldsymbol{O}.$$

Note that this is a special case of the testing problem (2) under the model (1). It holds that

$$c_{ij} = \frac{\sqrt{N_i N_j}}{N}\eta_{ij}, \quad i, j \in [\![g]\!].$$

After a simple calculation, it holds that $T_{\mathrm{ZGZ}} \equiv \mathrm{tr}(\boldsymbol{X}'\boldsymbol{\Omega}\boldsymbol{X})/N = T/N$ and $\hat{\sigma}^2_{\mathrm{ZGZ}} \equiv \hat{\sigma}^2_0/N^2$, where $\boldsymbol{\Omega}$ is given by (17) with $\boldsymbol{B} = \boldsymbol{R} = \boldsymbol{I}_p$. Consequently,

$$\frac{T_{\mathrm{ZGZ}}}{\sqrt{\hat{\sigma}^2_{\mathrm{ZGZ}}}} \equiv \frac{T}{\sqrt{\hat{\sigma}^2_0}}.$$

*S4.3. Test for two-way MANOVA*

In two-way MANOVA, we consider the treatments for the combinations of the levels of two factors, A and B, with factor levels $\mathrm{A}_1, \ldots, \mathrm{A}_a$ and $\mathrm{B}_1, \ldots, \mathrm{B}_b$, respectively, yielding a total of $ab$ treatments, where $a$ and $b$ satisfy $(a-1)(b-1) \geq 1$. Suppose that a $p$-dimensional random sample of size $N_{ij}$ is available from the $(i,j)$-th treatment group for $i \in [\![a]\!]$ and $j \in [\![b]\!]$. Let $\boldsymbol{x}_{ij1}, \ldots, \boldsymbol{x}_{ijN_{ij}}$ be $N_{ij}$ independent $p$-dimensional observation vectors obtained from the $(i,j)$-th treatment group. The model for each observation is given as follows:

$$\boldsymbol{x}_{ijk} = \boldsymbol{\eta}_{ij} + \boldsymbol{\varepsilon}_{ijk}, \quad i \in [\![a]\!], \quad j \in [\![b]\!], \quad k \in [\![N_{ij}]\!],$$

where $\boldsymbol{\eta}_{ij}$ denotes the mean for the $(i,j)$-th treatment group, $\boldsymbol{\varepsilon}_{ijk}$ is the error vector distributed as a $p$-dimensional distribution $F$ with mean $\mathbf{0}$ and covariance matrix $\boldsymbol{\Sigma}_{ij}$, and $F$ satisfies D1 and D2. We assume a two-way unbalanced MANOVA model with unequal covariance matrices; that is, we do not assume that

$$N_{11} = N_{12} = \cdots = N_{1b} = N_{21} = \cdots = N_{2b} = \cdots = N_{a1} = \cdots = N_{ab}, \tag{23}$$

$$\boldsymbol{\Sigma}_{11} = \boldsymbol{\Sigma}_{12} = \cdots = \boldsymbol{\Sigma}_{1b} = \boldsymbol{\Sigma}_{21} = \cdots = \boldsymbol{\Sigma}_{2b} = \cdots = \boldsymbol{\Sigma}_{a1} = \cdots = \boldsymbol{\Sigma}_{ab}. \tag{24}$$

Consider the following decomposition of $\boldsymbol{\eta}_{ij}$:

$$\boldsymbol{\eta}_{ij} = \boldsymbol{\mu} + \boldsymbol{\alpha}_i + \boldsymbol{\beta}_j + \boldsymbol{\gamma}_{ij}, \tag{25}$$

where $\boldsymbol{\mu}$ is the general mean, $\boldsymbol{\alpha}_i$ is an effect of the $i$-th level of factor A, $\boldsymbol{\beta}_j$ is an effect of the $j$-th level of factor B, and $\boldsymbol{\gamma}_{ij}$ represents an effect of the interaction between the factor level $\mathrm{A}_i$ and the factor level $\mathrm{B}_j$. To define $\boldsymbol{\mu}$, $\boldsymbol{\alpha}_i$, $\boldsymbol{\beta}_j$, and $\boldsymbol{\gamma}_{ij}$ uniquely, we impose the following constraints (see Fujikoshi et al. [3]):

$$\sum_{i=1}^{a} N_{i\cdot}\boldsymbol{\alpha}_i = \mathbf{0}, \quad \sum_{j=1}^{b} N_{\cdot j}\boldsymbol{\beta}_j = \mathbf{0}, \quad \sum_{i=1}^{a} N_{ij}\boldsymbol{\gamma}_{ij} = \mathbf{0}, \quad \sum_{j=1}^{b} N_{ij}\boldsymbol{\gamma}_{ij} = \mathbf{0}, \tag{26}$$

where

$$N_{i\cdot} = \sum_{j=1}^{b} N_{ij}, \quad i \in [\![a]\!]; \quad N_{\cdot j} = \sum_{i=1}^{a} N_{ij}, \quad j \in [\![b]\!].$$

This constraint was also used by Ananda and Weerahandi [1] for a two-way ANOVA analysis with unequal cell frequencies and unequal variances.

Under the constraint (26), consider the following testing hypotheses without assuming (24):

$$\begin{aligned} &H_\alpha : \boldsymbol{\alpha}_i = \mathbf{0} \text{ for } \forall i \in [\![a]\!]; \\ &H_\beta : \boldsymbol{\beta}_j = \mathbf{0} \text{ for } \forall j \in [\![b]\!]; \\ &H_\gamma : \boldsymbol{\gamma}_{ij} = \mathbf{0} \text{ for } \forall i \in [\![a]\!] \text{ and } \forall j \in [\![b]\!]. \end{aligned}$$

Let

$$\begin{aligned} \boldsymbol{X} = (&\boldsymbol{x}_{111}, \ldots, \boldsymbol{x}_{11N_{11}}, \ldots, \boldsymbol{x}_{1b1}, \ldots, \boldsymbol{x}_{1bN_{1b}}, \boldsymbol{x}_{211}, \ldots, \boldsymbol{x}_{21N_{21}}, \ldots, \boldsymbol{x}_{2b1}, \ldots, \boldsymbol{x}_{2bN_{2b}}, \\ &\ldots, \boldsymbol{x}_{a11}, \ldots, \boldsymbol{x}_{a1N_{a1}}, \ldots, \boldsymbol{x}_{ab1}, \ldots, \boldsymbol{x}_{abN_{ab}})'. \end{aligned} \tag{27}$$

Then,

$$\boldsymbol{X} = \boldsymbol{A}\boldsymbol{\Theta} + \boldsymbol{\mathcal{E}},$$

where

$$\begin{aligned} &\boldsymbol{A} = \mathrm{diag}(\mathbf{1}_{N_{11}}, \mathbf{1}_{N_{12}}, \ldots, \mathbf{1}_{N_{1b}}, \mathbf{1}_{N_{21}}, \ldots, \mathbf{1}_{N_{ab}}), \\ &\boldsymbol{\Theta} = (\boldsymbol{\eta}_{11}, \boldsymbol{\eta}_{12}, \ldots, \boldsymbol{\eta}_{1b}, \boldsymbol{\eta}_{21}, \ldots, \boldsymbol{\eta}_{2b}, \ldots, \boldsymbol{\eta}_{a1}, \ldots, \boldsymbol{\eta}_{ab})', \\ &\boldsymbol{\mathcal{E}} = (\boldsymbol{\varepsilon}_{111}, \ldots, \boldsymbol{\varepsilon}_{11N_{11}}, \ldots, \boldsymbol{\varepsilon}_{1b1}, \ldots, \boldsymbol{\varepsilon}_{1bN_{1b}}, \boldsymbol{\varepsilon}_{211}, \ldots, \boldsymbol{\varepsilon}_{21N_{21}}, \ldots, \boldsymbol{\varepsilon}_{2b1}, \ldots, \boldsymbol{\varepsilon}_{2bN_{2b}}, \\ &\qquad \ldots, \boldsymbol{\varepsilon}_{a11}, \ldots, \boldsymbol{\varepsilon}_{a1N_{a1}}, \ldots, \boldsymbol{\varepsilon}_{ab1}, \ldots, \boldsymbol{\varepsilon}_{abN_{ab}})'. \end{aligned}$$

First, we propose the criterion for testing the null hypothesis $H_\alpha$, which can be applied even when $p > N_{ij}$ for $i \in [\![a]\!]$ and $j \in [\![b]\!]$. Define

$$\boldsymbol{G}_1 = \boldsymbol{A}(\boldsymbol{I}_a \otimes \mathbf{1}_b), \quad \boldsymbol{G}_2 = \boldsymbol{A}(\mathbf{1}_a \otimes \boldsymbol{I}_b), \quad \boldsymbol{G}_3 = \boldsymbol{A}.$$

Then,

$$\boldsymbol{X} = \boldsymbol{G}\boldsymbol{\Xi} + \boldsymbol{\mathcal{E}}, \tag{28}$$

where

$$\begin{aligned} &\boldsymbol{G} = (\mathbf{1}_N, \boldsymbol{G}_1, \boldsymbol{G}_2, \boldsymbol{G}_3), \\ &\boldsymbol{\Xi} = (\boldsymbol{\mu}, \boldsymbol{\mathcal{A}}', \boldsymbol{\mathcal{B}}', \boldsymbol{\Gamma}')', \\ &\boldsymbol{\mathcal{A}} = (\boldsymbol{\alpha}_1, \ldots, \boldsymbol{\alpha}_a)', \quad \boldsymbol{\mathcal{B}} = (\boldsymbol{\beta}_1, \ldots, \boldsymbol{\beta}_b)', \quad \boldsymbol{\Gamma} = (\boldsymbol{\gamma}_{11}, \ldots, \boldsymbol{\gamma}_{1b}, \ldots, \boldsymbol{\gamma}_{a1}, \ldots, \boldsymbol{\gamma}_{ab})'. \end{aligned}$$

The constraint (26) can be described as follows:

$$\mathbf{1}_N'\boldsymbol{G}_1\boldsymbol{\mathcal{A}} = \boldsymbol{O}, \quad \mathbf{1}_N'\boldsymbol{G}_2\boldsymbol{\mathcal{B}} = \boldsymbol{O}, \quad (\boldsymbol{G}_1, \boldsymbol{G}_2)'\boldsymbol{G}_3\boldsymbol{\Gamma} = \boldsymbol{O}, \tag{29}$$

where $N = N_{\cdot\cdot} = \sum_{i=1}^a N_{i\cdot} = \sum_{j=1}^b N_{\cdot j}$. Then, the null hypothesis $H_\alpha : \boldsymbol{\alpha}_i = \mathbf{0}, \forall i \in [\![a]\!]$ under the model (25) with the constraint (26) is equivalent to the null hypothesis $H_\alpha : \boldsymbol{L}\boldsymbol{\Theta} = \boldsymbol{O}$ under the model

(25) with the constraint (29), where $\boldsymbol{L} = \boldsymbol{\mathcal{K}}'\boldsymbol{A}$ is an $(a-1) \times ab$ matrix, $\boldsymbol{\mathcal{K}}$ is an $N \times (a-1)$ matrix such that $\boldsymbol{\mathcal{K}}'\boldsymbol{\mathcal{K}} = \boldsymbol{I}_{a-1}$, and

$$\boldsymbol{\mathcal{K}}\boldsymbol{\mathcal{K}}' = \boldsymbol{\Pi}_{(\boldsymbol{G}_1,\boldsymbol{G}_2)} - \boldsymbol{\Pi}_{\boldsymbol{G}_2} = \boldsymbol{\Pi}_{\boldsymbol{A}} - \{\boldsymbol{\Pi}_{\boldsymbol{1}_N} + (\boldsymbol{\Pi}_{\boldsymbol{G}_2} - \boldsymbol{\Pi}_{\boldsymbol{1}_N}) + (\boldsymbol{\Pi}_{\boldsymbol{A}} - \boldsymbol{\Pi}_{(\boldsymbol{G}_1,\boldsymbol{G}_2)})\},$$

$$\boldsymbol{\Pi}_{(\boldsymbol{G}_1\boldsymbol{G}_2)} = (\boldsymbol{G}_1, \boldsymbol{G}_2)\begin{pmatrix} \boldsymbol{G}_1'\boldsymbol{G}_1 & \boldsymbol{G}_1'\boldsymbol{G}_2 \\ \boldsymbol{G}_2'\boldsymbol{G}_1 & \boldsymbol{G}_2'\boldsymbol{G}_2 \end{pmatrix}^+ (\boldsymbol{G}_1, \boldsymbol{G}_2)', \quad \boldsymbol{\Pi}_{\boldsymbol{G}_2} = \boldsymbol{G}_2(\boldsymbol{G}_2'\boldsymbol{G}_2)^{-1}\boldsymbol{G}_2'.$$

For further details, please refer to Fujikoshi et al. [3]. Note that $(\boldsymbol{G}_1, \boldsymbol{G}_2)'(\boldsymbol{G}_1, \boldsymbol{G}_2)$ becomes singular because $\mathrm{rank}((\boldsymbol{G}_1, \boldsymbol{G}_2)) = a + b - 1$. Thus, we use the Moore-Penrose inverse of $(\boldsymbol{G}_1, \boldsymbol{G}_2)'(\boldsymbol{G}_1, \boldsymbol{G}_2)$ to define $\boldsymbol{\Pi}_{(\boldsymbol{G}_1,\boldsymbol{G}_2)}$. Accordingly,

$$\boldsymbol{\Pi}_{\mathrm{H}_\alpha} = \boldsymbol{\Pi}_{\boldsymbol{A}}\boldsymbol{\mathcal{K}}(\boldsymbol{\mathcal{K}}'\boldsymbol{\Pi}_{\boldsymbol{A}}\boldsymbol{\mathcal{K}})^{-1}\boldsymbol{\mathcal{K}}'\boldsymbol{\Pi}_{\boldsymbol{A}} = \boldsymbol{\Pi}_{(\boldsymbol{G}_1,\boldsymbol{G}_2)} - \boldsymbol{\Pi}_{\boldsymbol{G}_2}, \tag{30}$$

where the last equality can be derived from $\boldsymbol{\mathcal{K}}'\boldsymbol{\Pi}_{\boldsymbol{A}} = \boldsymbol{\mathcal{K}}'$. Let

$$\begin{aligned} \boldsymbol{d}_\alpha &= \{(\boldsymbol{I}_N - \boldsymbol{\Pi}_{\boldsymbol{A}}) \odot (\boldsymbol{I}_N - \boldsymbol{\Pi}_{\boldsymbol{A}})\}^{-1}(h_{\alpha,11}, \ldots, h_{\alpha,NN})' \\ &= \mathrm{diag}\,(\boldsymbol{M}_{11}, \ldots, \boldsymbol{M}_{1b}, \ldots, \boldsymbol{M}_{a1}, \ldots, \boldsymbol{M}_{ab})\,(h_{\alpha,11}, \ldots, h_{\alpha,NN})', \end{aligned} \tag{31}$$

where $(h_{\alpha,ij}) = \boldsymbol{\Pi}_{\mathrm{H}_\alpha}$ and

$$\boldsymbol{M}_{ij} = \frac{N_{ij}}{N_{ij} - 2}\left(\boldsymbol{I}_{N_{ij}} - \frac{1}{N_{ij} - 1}\boldsymbol{\Pi}_{N_{ij}}\right), \quad i \in [\![a]\!], \quad j \in [\![b]\!].$$

From (30) and (31), we obtain the testing statistic as $T_\alpha = \mathrm{tr}(\boldsymbol{X}'\boldsymbol{\Omega}_\alpha\boldsymbol{X})$, where

$$\boldsymbol{\Omega}_\alpha = \boldsymbol{\Pi}_{\mathrm{H}_\alpha} - (\boldsymbol{I}_N - \boldsymbol{\Pi}_{\boldsymbol{A}})\mathrm{diag}(\boldsymbol{d}_\alpha)(\boldsymbol{I}_N - \boldsymbol{\Pi}_{\boldsymbol{A}}).$$

Using the same method of derivation, the statistics for testing the null hypotheses $H_\beta$ and $H_\gamma$ are obtained as $T_\beta = \mathrm{tr}(\boldsymbol{X}'\boldsymbol{\Omega}_\beta\boldsymbol{X})$ and $T_\gamma = \mathrm{tr}(\boldsymbol{X}'\boldsymbol{\Omega}_\gamma\boldsymbol{X})$, respectively, where

$$\begin{aligned} &\boldsymbol{\Omega}_\beta = \boldsymbol{\Pi}_{\mathrm{H}_\beta} - (\boldsymbol{I}_N - \boldsymbol{\Pi}_{\boldsymbol{A}})\mathrm{diag}(\boldsymbol{d}_\beta)(\boldsymbol{I}_N - \boldsymbol{\Pi}_{\boldsymbol{A}}), \quad \boldsymbol{\Omega}_\gamma = \boldsymbol{\Pi}_{\mathrm{H}_\gamma} - (\boldsymbol{I}_N - \boldsymbol{\Pi}_{\boldsymbol{A}})\mathrm{diag}(\boldsymbol{d}_\gamma)(\boldsymbol{I}_N - \boldsymbol{\Pi}_{\boldsymbol{A}}), \\ &\boldsymbol{\Pi}_{\mathrm{H}_\beta} = \boldsymbol{\Pi}_{(\boldsymbol{G}_1,\boldsymbol{G}_2)} - \boldsymbol{\Pi}_{\boldsymbol{G}_1}, \quad \boldsymbol{\Pi}_{\mathrm{H}_\gamma} = \boldsymbol{\Pi}_{\boldsymbol{A}} - \boldsymbol{\Pi}_{(\boldsymbol{G}_1,\boldsymbol{G}_2)}, \\ &\boldsymbol{d}_\beta = \{(\boldsymbol{I}_N - \boldsymbol{\Pi}_{\boldsymbol{A}}) \odot (\boldsymbol{I}_N - \boldsymbol{\Pi}_{\boldsymbol{A}})\}^{-1}(h_{\beta,11}, \ldots, h_{\beta,NN})', \\ &\boldsymbol{d}_\gamma = \{(\boldsymbol{I}_N - \boldsymbol{\Pi}_{\boldsymbol{A}}) \odot (\boldsymbol{I}_N - \boldsymbol{\Pi}_{\boldsymbol{A}})\}^{-1}(h_{\gamma,11}, \ldots, h_{\gamma,NN})' \end{aligned}$$

for $(h_{\beta,ij}) = \boldsymbol{\Pi}_{\mathrm{H}_\beta}$ and $(h_{\gamma,ij}) = \boldsymbol{\Pi}_{\mathrm{H}_\gamma}$.

To construct the testing criterion, we propose a consistent estimator of the asymptotic variance of the testing statistic. The asymptotic variance $\sigma_\alpha^2$ of $T_\alpha$ is given by $2\,\mathrm{tr}((\boldsymbol{\Omega}_\alpha \odot \boldsymbol{\Omega}_\alpha)\boldsymbol{V}_{ab})$, where $\boldsymbol{V}_{ab}$ has the same structure as that in (7), i.e., the $(ij, ij)$-th block is defined by $a_{ij,2}\boldsymbol{1}_{N_{ij}}\boldsymbol{1}_{N_{ij}}'$ and the $(ij, k\ell)$-th block is defined by $b_{ij,k\ell}\boldsymbol{1}_{N_{ij}}\boldsymbol{1}_{N_{k\ell}}'$ for $(i,j) \neq (k,\ell)$. In addition, the indices of the blocks required for

constructing $\boldsymbol{V}_{ab}$ are ordered as

$$(1,1) \succ (1,2) \succ \cdots \succ (1,b) \succ (2,1) \succ \cdots \succ (2,b) \succ \cdots \succ (a,1) \succ \cdots \succ (a,b).$$

The consistent estimator $\hat{\sigma}_\alpha^2$ of $\sigma_\alpha^2$ is obtained by replacing the unknown parameters with their consistent estimators, i.e., $\hat{\sigma}_\alpha^2 = 2\,\mathrm{tr}((\boldsymbol{\Omega}_\alpha \odot \boldsymbol{\Omega}_\alpha)\hat{\boldsymbol{V}}_{ab})$; in addition, $\hat{\boldsymbol{V}}_{ab}$ is obtained by replacing $a_{ij,2}$ and $b_{ij,k\ell}$ in $\boldsymbol{V}_{ab}$ with their consistent estimators, which are given as follows:

$$\hat{a}_{ij,2} = \frac{N_{ij}-1}{N_{ij}(N_{ij}-2)(N_{ij}-3)} \left\{(N_{ij}-1)(N_{ij}-2)\,\mathrm{tr}(\boldsymbol{S}_{ij}^2) + (\mathrm{tr}(\boldsymbol{S}_{ij}))^2 - N_{ij}Q_{ij}\right\}, \quad (i,j) \in \boldsymbol{J}_{ab},$$
$$\hat{b}_{ij,k\ell} = \mathrm{tr}(\boldsymbol{S}_{ij}\boldsymbol{S}_{k\ell}), \quad (i,j),(k,\ell) \in \boldsymbol{J}_{ab}, \quad (i,j) \neq (k,\ell),$$

where

$$\boldsymbol{J}_{ab} = \{(i,j) \mid i \in [\![a]\!],\ j \in [\![b]\!]\}.$$

Here,

$$\boldsymbol{S}_{ij} = \frac{1}{N_{ij}-1}\sum_{j=1}^{N_{ij}}(\boldsymbol{x}_{ijk} - \bar{\boldsymbol{x}}_{ij})(\boldsymbol{x}_{ijk} - \bar{\boldsymbol{x}}_{ij})', \quad Q_{ij} = \frac{1}{N_{ij}-1}\sum_{k=1}^{N_{ij}}\left\{(\boldsymbol{x}_{ijk} - \bar{\boldsymbol{x}}_{ij})'(\boldsymbol{x}_{ijk} - \bar{\boldsymbol{x}}_{ij})\right\}^2.$$

Using the same derivation method, we can derive the consistent estimators $\hat{\sigma}_\beta^2$ and $\hat{\sigma}_\gamma^2$ of the asymptotic variances $\sigma_\beta^2$ and $\sigma_\gamma^2$ of $T_\beta$ and $T_\gamma$, respectively, which are defined as follows:

$$\hat{\sigma}_\beta^2 = 2\,\mathrm{tr}((\boldsymbol{\Omega}_\beta \odot \boldsymbol{\Omega}_\beta)\hat{\boldsymbol{V}}_{ab}), \quad \hat{\sigma}_\gamma^2 = 2\,\mathrm{tr}((\boldsymbol{\Omega}_\gamma \odot \boldsymbol{\Omega}_\gamma)\hat{\boldsymbol{V}}_{ab}).$$

Note that $\hat{\sigma}_\alpha^2$, $\hat{\sigma}_\beta^2$, and $\hat{\sigma}_\gamma^2$ do not take negative values with probability 1. The proposed testing criterion for testing the null hypothesis $H_*$, where $*$ can be $\alpha$, $\beta$, or $\gamma$, with the significance level $\varepsilon$, and without assuming (23) or (24), is as follows. For the observation matrix $\boldsymbol{X}$ given by (27),

$$\frac{T_*}{\sqrt{\hat{\sigma}_*^2}} > \Phi^{-1}(1-\varepsilon) \quad \Longrightarrow \quad \text{Reject the null hypothesis } H_*. \tag{32}$$

*S4.4. Test for parallelism in profile analysis*

Profile analysis is an example of testing the bilateral linear hypothesis (2) under the generalized multivariate linear model (1) (see Srivastava [6]). We use the same model as that presented in Section S4.1, i.e., we use the design matrix $\boldsymbol{A}$ defined in (9) along with the design matrix $\boldsymbol{B}$ and mean matrix $\boldsymbol{\Theta}$ defined in (16).

For the parallelism of the mean vectors,

$$H_{\mathrm{p},0} : \boldsymbol{\mu}_i - \boldsymbol{\mu}_g = \gamma_i \boldsymbol{1}_p, \quad \gamma_i \in \mathbb{R}, \quad \forall i \in [\![g-1]\!] \iff H_{\mathrm{p},0} : \boldsymbol{L\Theta R} = \boldsymbol{O},$$

where $\boldsymbol{L}$ is defined as (20) and $\boldsymbol{R} = (\boldsymbol{I}_{p-1}, -\boldsymbol{1}_{p-1})$. In this case, $\boldsymbol{\Omega}$ has the same structure as that in

(17), and $\eta_{ij}$ is given by (21), $\boldsymbol{\mathcal{P}} = (\boldsymbol{R}'\boldsymbol{R})^{-1/2}\boldsymbol{R}$; thus, $T = \mathrm{tr}(\boldsymbol{\mathcal{P}}\boldsymbol{X}'\boldsymbol{\Omega}\boldsymbol{X}\boldsymbol{\mathcal{P}}')$ can be described as

$$\begin{aligned}
&\mathrm{tr}(\boldsymbol{\mathcal{P}}\boldsymbol{X}'\boldsymbol{\Pi}_{\mathrm{H}}\boldsymbol{X}\boldsymbol{\mathcal{P}}') - \mathrm{tr}(\boldsymbol{\mathcal{P}}\boldsymbol{X}'(\boldsymbol{I}_N - \boldsymbol{\Pi}_{\mathrm{A}})\boldsymbol{D}(\boldsymbol{I}_N - \boldsymbol{\Pi}_{\mathrm{A}})\boldsymbol{X}\boldsymbol{\mathcal{P}}') \\
&= \mathrm{tr}(\boldsymbol{\Pi}_{\mathrm{H}}\boldsymbol{X}\boldsymbol{\mathcal{P}}'\boldsymbol{\mathcal{P}}\boldsymbol{X}'\boldsymbol{\Pi}_{\mathrm{H}}) - \mathrm{tr}\left(\boldsymbol{D}(\boldsymbol{I}_N - \boldsymbol{\Pi}_{\mathrm{A}})\boldsymbol{X}\boldsymbol{\mathcal{P}}'\boldsymbol{\mathcal{P}}\boldsymbol{X}'(\boldsymbol{I}_N - \boldsymbol{\Pi}_{\mathrm{A}})\right) \\
&= \mathrm{tr}(\boldsymbol{\Pi}_{\mathrm{H}}\boldsymbol{X}\boldsymbol{\Pi}_{\boldsymbol{R}}\boldsymbol{X}'\boldsymbol{\Pi}_{\mathrm{H}}) - \sum_{i=1}^{g} \frac{1 - N_i/N}{N_i - 1}(N_i - 1)\,\mathrm{tr}(\bar{\boldsymbol{S}}_i) \\
&= \mathrm{tr}(\bar{\boldsymbol{S}}_{\mathrm{h}}) - \sum_{i=1}^{g}\left(1 - \frac{N_i}{N}\right)\mathrm{tr}(\bar{\boldsymbol{S}}_i) = T_{\mathrm{p}},
\end{aligned}$$

where $\bar{\boldsymbol{S}}_{\mathrm{h}} = \boldsymbol{\Pi}_{\boldsymbol{R}}\boldsymbol{S}_{\mathrm{h}}\boldsymbol{\Pi}_{\boldsymbol{R}}$, $\bar{\boldsymbol{S}}_i = \boldsymbol{\Pi}_{\boldsymbol{R}}\boldsymbol{S}_i\boldsymbol{\Pi}_{\boldsymbol{R}}$, $\boldsymbol{S}_{\mathrm{h}}$ and $\boldsymbol{S}_i$ are defined in (22) and (19), respectively, and $\boldsymbol{\Pi}_{\boldsymbol{R}} = \boldsymbol{R}'(\boldsymbol{R}\boldsymbol{R}')^{-1}\boldsymbol{R} = \boldsymbol{I}_p - \frac{1}{p}\boldsymbol{1}_p\boldsymbol{1}_p'$. The proposed criterion for testing the null hypothesis $H_{p,0}$ : $\boldsymbol{\mu}_i - \boldsymbol{\mu}_g = \gamma_i\boldsymbol{1}_p$, $\gamma_i \in \mathbb{R}$, $\forall i \in [\![g-1]\!]$, with significance level $\varepsilon$ is as follows:

$$\frac{T_{\mathrm{p}}}{\sqrt{\hat{\sigma}_{\mathrm{p}}^2}} > \Phi^{-1}(1-\varepsilon) \quad \Longrightarrow \quad \text{Reject the null hypothesis } H_{\mathrm{p},0},$$

where $\hat{\sigma}_{\mathrm{p}}^2$ is the same as $\hat{\sigma}_0^2$ given in (18).

## S5. Numerical study

This section presents the results of the numerical experiments designed to evaluate the performance of the proposed test for a finite sample in terms of size control and power. Specifically, by focusing on the robustness to violate the assumptions of normality and homoscedasticity, we conduct simulations for various population distributions in combination with several covariance structures. To illustrate the application of our results, we also employ the proposed test to investigate energy homeostasis in mammals, specifically to analyze the effect of fasting on the gene expression profiles in various tissues using the DNA microarray data.

### *S5.1. Simulation results*

Owing to their high practicality, we report the numerical results for two-way MANOVA. For other examples of the proposed class of statistics, our simulation results are found to correspond with those reported in the literature for each specific test; please refer to Chen and Qin [2], Yamada and Himeno [7], and Zhou et al. [8] (whose results are not included herein).

We assume a multivariate linear model (28) and set $a = 2$ and $b = 3$ for the numbers of levels of A and B, respectively. We restrict the presentation for testing the hypotheses

$$H_\alpha : \boldsymbol{\alpha}_i = \boldsymbol{0}, \quad \forall i \in \{1,2\} \quad \text{and} \quad H_\gamma : \boldsymbol{\gamma}_{ij} = \boldsymbol{0}, \quad \forall i \in \{1,2\}, \quad \forall j \in \{1,2,3\}. \tag{33}$$

Testing of $H_\beta : \boldsymbol{\beta}_j = \boldsymbol{0}, \forall j \in \{1,2,3\}$ can be conducted using similar fashion, of which the results are omitted here, owing to lack of space.

In what follows, we summarize the data-generating mechanism, starting with the parameter setting.

*Construction of $\boldsymbol{\mathcal{A}}$.*

1. We set a $p \times a$ matrix $\Xi_1 = (\boldsymbol{\xi}_1, \dots, \boldsymbol{\xi}_a)$, where $\boldsymbol{\xi}_i = (\delta/256)p^{\delta/256}\boldsymbol{e}_i$ and $\boldsymbol{e}_i$ is a unit vector with the $i$th position being 1.
2. Set $\Xi_2 = \Xi_1 \operatorname{diag}(N_{1\cdot}/N, \dots, N_{a\cdot}/N)$.
3. Set $\boldsymbol{\xi}$ as the sum of the column vectors of $\Xi_2$.
4. Set $\boldsymbol{\mathcal{A}} = (\Xi_1 - (\boldsymbol{\xi}, \dots, \boldsymbol{\xi}))'$.

*Construction of $\boldsymbol{\Gamma}$.*

1. Set a $p \times b$ matrix $\Xi_1 = (\boldsymbol{\xi}_1, \dots, \boldsymbol{\xi}_b)$, where $\boldsymbol{\xi}_i = (\delta/256)p^{\delta/256}\boldsymbol{e}_i$.
2. Set $\Xi_2 = \Xi_1 \operatorname{diag}(N_{11}/N_{1\cdot}, \dots, N_{1b}/N_{1\cdot})$.
3. Set $\boldsymbol{\xi}$ as the sum of the column vectors of $\Xi_2$.
4. Set $\Xi_3 = \Xi_1 - (\boldsymbol{\xi}, \dots, \boldsymbol{\xi})$.
5. Set $\Xi_4^{(i)} = \Xi_3 \operatorname{diag}(N_{11}/N_{i1}, \dots, N_{1b}/N_{ib})$ for $i = 2, \dots, a$.
6. Set $\boldsymbol{\Gamma} = (\Xi_3, -\Xi_4^{(2)}/(a-1), \dots, -\Xi_4^{(a)}/(a-1))'$.

*Construction of $\boldsymbol{\mathcal{B}}$.*

1. Set a $p \times b$ matrix $\Xi_1$ whose elements are generated from the independent random numbers distributed as $N(0, 1)$.
2. Set $\Xi_2 = \Xi_1 \operatorname{diag}(N_{\cdot 1}/N, \dots, N_{\cdot b}/N)$.
3. Set $\boldsymbol{\xi}$ as the sum of column vectors of $\Xi_2$.
4. Set $\boldsymbol{\mathcal{B}} = (\Xi_1 - (\boldsymbol{\xi}, \dots, \boldsymbol{\xi}))'$.

This parametrization satisfies the constraints (26), guaranteeing the uniqueness of the definition of $\boldsymbol{\alpha}_i$ and $\boldsymbol{\gamma}_{ij}$. For the dimensions, we take the values $p \in \{200, 400, 800, 1200\}$; for $a = 2$ and $b = 3$, we use $(N_{11}, N_{12}, N_{13}, N_{21}, N_{22}, N_{23}) = (11, 12, 13, 14, 15, 16)$, which corresponds to a high-dimensional and unbalanced setup; and we take $\delta \in \{0, 60, 75, 90, 105\}$. Furthermore, we consider the following settings for the distribution $F$ of $\boldsymbol{z}_i, \dots, \boldsymbol{z}_N$ in (8).

- F1: $F$ is a $p$-dimensional normal distribution with mean $\mathbf{0}$ and covariance matrix $\boldsymbol{I}_p$.
- F2: $F$ is a standardized $p$-dimensional $t$ distribution with 10 degrees of freedom.
- F3: $F$ is a standardized $p$-dimensional zero-mean contaminated normal distribution with mixing probability 0.1 and contamination parameter 3.
- F4: $F$ is a $p$-dimensional distribution whose univariate marginals are independently standardized, chi-squared distributions with 10 degrees of freedom.

Distributions F1-F4 satisfy the conditions D1 and D2 of the asymptotic theory (see Section 3) and are included to investigate the violation of the normality assumption. For each distribution, we use three covariance structures of $\boldsymbol{\Sigma}_{ij}$ in (8) for the $i$-th factor of level A and $j$-th factor of level B of the $p$-variate observation vector

- M1: $\boldsymbol{\Sigma}_{ij} = \boldsymbol{I}_p$.

M2: $\boldsymbol{\Sigma}_{ij} = \boldsymbol{D}\boldsymbol{\mathcal{R}}^{(ij)}\boldsymbol{D}$, where $\boldsymbol{D}$ is a $p$-dimensional diagonal matrix whose $i$-th diagonal element is given by $2 + (p - i + 1)/p$, and $\boldsymbol{\mathcal{R}}^{(ij)} = (\rho_{k\ell}^{(ij)})$ is a $p$-dimensional symmetric matrix where the $(k, \ell)$ element of $\boldsymbol{\mathcal{R}}^{(ij)}$ is given by

$$\rho_{k\ell}^{(ij)} = (-1)^{k+\ell} \left\{ \frac{i+j}{10(a+b)} \right\}^{|k-\ell|/7}.$$

M3: Generate a sparse positive-definite matrix as $\boldsymbol{\Sigma}_{ij}$ by using the following algorithm: with sparsity parameter $s = 0.7$.

**Algorithm**: Generate sparse covariance matrix $\boldsymbol{\Sigma}_{ij}$

1: Construct $p$-dimensional symmetric matrix $\boldsymbol{\mathcal{R}}^{(ij)} = (\rho_{k\ell}^{(ij)})$ as follows

2: **for** $k < \ell$ **do**

$$\rho_{k\ell}^{(ij)} = \begin{cases} \text{Unif}(0,1) & \text{with probability } (1-s) \times 0.75, \\ \text{Unif}(-1,0) & \text{with probability } (1-s) \times 0.25, \\ 0 & \text{with probability } s, \end{cases}$$

where $s$ is the level of sparsity in $\boldsymbol{\mathcal{R}}^{(ij)}$.

3: **end for**

4: Set $\rho_{k\ell}^{(ij)} = \rho_{\ell k}^{(ij)}$ to obtain the symmetry and diagonal elements of $\boldsymbol{\mathcal{R}}^{(ij)}$ to equal 1.

5: To obtain the positive definiteness of $\boldsymbol{\Sigma}_{ij}$, calculate the minimum eigenvalue $e_{\min}$ of $\boldsymbol{\mathcal{R}}^{(ij)}$. Set

$$\boldsymbol{R}^{(ij)} = \begin{cases} \boldsymbol{\mathcal{R}} + (-e_{\min} + 0.1)\boldsymbol{I}_p & \text{if } e_{\min} \leq 0, \\ \boldsymbol{\mathcal{R}} & \text{otherwise.} \end{cases}$$

6: $\boldsymbol{\Sigma}_{ij} = \boldsymbol{D}\text{diag}(\boldsymbol{R}^{(ij)})^{-1/2}\boldsymbol{R}^{(ij)}\text{diag}(\boldsymbol{R}^{(ij)})^{-1/2}\boldsymbol{D}$, where $\boldsymbol{D} = (d_{ij})$ is a $p$-dimensional diagonal matrix such that $d_{11}, \ldots, d_{pp}$ have an i.i.d. chi-squared distribution with 1 degree of freedom.

Both M2 and M3 are included to illustrate the violation of the assumed homoscedasticity. It should also be noted that $\boldsymbol{\Omega}_\alpha$, $\boldsymbol{\Omega}_\beta$, and $\boldsymbol{\Omega}_\gamma$ satisfy A1; see Section 3. In addition, the models M1 and M2 satisfy A2 (see Yamada and Himeno [7]), but M3 does not.

We assess the accuracy of the tests given in (32) for $* = \alpha, \gamma$. Targeting the nominal size of $\varepsilon = 0.05$, the null hypotheses (33) are rejected when the observed values of the testing statistics exceed the $1 - \varepsilon = 0.95$ percentile of a standard normal distribution. We generate the data under the null hypotheses $H_\alpha$ and $H_\gamma$, using $10,000$ simulation runs for each combination of $p$ and $N_i$, four distributions, and three covariance structures; we carry out by setting $\delta = 0$ during the construction of $\boldsymbol{\mathcal{A}}$ and $\boldsymbol{\Gamma}$. The attained significance levels of $T_\alpha$ and $T_\gamma$ are summarized in Table 1.

For both $T_\alpha/\hat{\sigma}_\alpha$ and $T_\gamma/\hat{\sigma}_\gamma$, we observe an accurate size control within 0.01 from the nominal significance level in high dimensions in almost all cases and across all covariance structures, in combination with all types of distributions. As expected, the sizes of the tests generally get close to the nominal level as $p$ increases, indicating that the asymptotic property of $T$ described in Theorem 3 pitches in. The accuracy of the distribution modeled by F4, as a non-normal case, is also important. Similarly, the covariance structures involving M2 and M3 are important as well. The former case models the *highly heteroscedastic* state with significantly different values of $\boldsymbol{\Sigma}_{ij}$ for different combinations of $(i, j)$,

Table 1: Attained significance levels (%) based on 10,000 simulation runs at the 0.05 nominal significance level.

| | $T_\alpha/\sqrt{\hat{\sigma}_\alpha}$ | | | | | | | | | | | |
|---|---|---|---|---|---|---|---|---|---|---|---|---|
| | M1 | | | | M2 | | | | M3 | | | |
| $p$ | F1 | F2 | F3 | F4 | F1 | F2 | F3 | F4 | F1 | F2 | F3 | F4 |
| 200 | 5.48 | 5.71 | 5.40 | 5.80 | 6.54 | 6.57 | 6.23 | 6.22 | 5.72 | 5.66 | 5.85 | 5.65 |
| 400 | 5.44 | 5.71 | 5.54 | 5.30 | 5.94 | 6.09 | 5.52 | 6.06 | 5.54 | 5.43 | 5.44 | 5.35 |
| 800 | 5.63 | 4.82 | 5.30 | 5.15 | 5.96 | 5.55 | 5.32 | 5.60 | 5.57 | 5.42 | 5.18 | 5.73 |
| 1200 | 5.15 | 5.09 | 4.87 | 5.31 | 5.83 | 5.83 | 5.10 | 5.43 | 5.30 | 5.77 | 5.25 | 5.27 |

| | $T_\gamma/\sqrt{\hat{\sigma}_\gamma}$ | | | | | | | | | | | |
|---|---|---|---|---|---|---|---|---|---|---|---|---|
| | M1 | | | | M2 | | | | M3 | | | |
| $p$ | F1 | F2 | F3 | F4 | F1 | F2 | F3 | F4 | F1 | F2 | F3 | F4 |
| 200 | 5.57 | 5.64 | 5.36 | 4.85 | 5.78 | 5.57 | 6.10 | 5.98 | 5.19 | 5.35 | 5.47 | 5.65 |
| 400 | 4.99 | 5.21 | 5.64 | 5.08 | 5.51 | 5.54 | 5.55 | 5.98 | 5.46 | 5.27 | 5.39 | 5.16 |
| 800 | 5.40 | 5.27 | 5.00 | 5.09 | 5.54 | 5.51 | 5.94 | 5.21 | 4.89 | 4.90 | 5.23 | 5.21 |
| 1200 | 5.21 | 5.07 | 5.21 | 5.26 | 5.44 | 5.30 | 5.61 | 5.59 | 5.27 | 5.06 | 5.49 | 5.15 |

whereas the latter case represents the most realistic situation under high dimensionality, i.e., a random structure with sparsity patterns that do not always satisfy assumption A2; however, our proposed test seems to work well. These numerical results demonstrate the strong robustness of the proposed class of tests against violations of typical assumptions.

Table 2 displays the empirical powers, where the power reaches 1 even for $\delta = 90$ in M1 for both $T_\alpha/\hat{\sigma}_\alpha$ and $T_\gamma/\hat{\sigma}_\gamma$. The power in M2 seems to be the lowest among the three cases, and increases with $p$ when $\delta = 90, 105$. This power increasing tendency is also observed in M3. We also report that the powers are almost the same in all distributions of F1-F4.

*S5.2. Example of real data applications*

We employ our proposed test to investigate the regulation of metabolic homeostasis in mammals, using the DNA microarray data presented by Nakai et al. [4], which are publicly available at the National Center for Biotechnology Information (NCBI) Gene Expression Omnibus, (`https://www.ncbi.nlm.nih.gov/geo/`), with the GEO Series ID GSE7623.

The data are obtained from a study on the effects of fasting on the gene expression profile in the ubiquitin-proteasome system of rats; this effect is involved in saving energy as an adaptation of mammals to food shortage. A DNA microarray analysis is conducted, and $p = 31,099$ gene expression profiles are automatically generated from three tissues, i.e., brown adipose tissue (BAT), white adipose tissue (WAT), and liver (LIV). The tissues are obtained from rats that have been either fed or fasted for 24 h. Because the functional balance among these three tissues is an important factor affecting the metabolic homeostasis, a specific goal of this study is to investigate the marginal and combined effects of food deprivation on the gene expression profiles of BAT, WAT, and LIV. Nakai et al. [4] applied four quantification methods to the raw data (Affymetrix CEL files) and considered the false discovery rate; to obtain more robust results, they recommended the selection of top-ranked genes common to all four datasets. Following the proposed ranking strategy, we focus on the $p = 1,000$ most informative genes for analyzing the data.

Table 2: Empirical powers (%) based on 10,000 simulation runs at the 0.05 nominal significance level.

| | | $T_\alpha/\sqrt{\hat{\sigma}_\alpha}$ | | | | | | | | | | | |
|---|---|---|---|---|---|---|---|---|---|---|---|---|---|
| | | M1 | | | | M2 | | | | M3 | | | |
| $p$ | $\delta$ | F1 | F2 | F3 | F4 | F1 | F2 | F3 | F4 | F1 | F2 | F3 | F4 |
| 200 | 60 | 32.8 | 33.0 | 34.0 | 33.1 | 7.7 | 7.4 | 7.4 | 7.5 | 8.1 | 8.3 | 8.4 | 8.1 |
| | 75 | 92.5 | 92.2 | 92.4 | 92.4 | 11.2 | 10.7 | 11.3 | 11.3 | 15.1 | 15.5 | 14.6 | 15.0 |
| | 90 | 100 | 100 | 100 | 100 | 23.5 | 24.1 | 23.3 | 22.9 | 41.0 | 40.9 | 39.7 | 41.4 |
| | 105 | 100 | 100 | 100 | 100 | 65.1 | 66.1 | 65.3 | 65.0 | 92.1 | 91.9 | 91.9 | 91.8 |
| 400 | 60 | 33.0 | 32.8 | 32.4 | 32.0 | 7.2 | 6.9 | 6.8 | 7.5 | 8.5 | 7.9 | 8.0 | 7.5 |
| | 75 | 95.5 | 95.6 | 95.4 | 95.6 | 11.3 | 10.7 | 11.2 | 11.4 | 15.2 | 15.1 | 15.5 | 14.6 |
| | 90 | 100 | 100 | 100 | 100 | 26.3 | 27.4 | 26.9 | 26.2 | 48.0 | 48.8 | 47.7 | 48.5 |
| | 105 | 100 | 100 | 100 | 100 | 81.3 | 81.8 | 80.3 | 81.5 | 98.4 | 98.4 | 98.4 | 98.4 |
| 800 | 60 | 30.6 | 31.9 | 31.9 | 31.7 | 7.4 | 6.9 | 6.7 | 6.9 | 7.9 | 7.9 | 8.0 | 7.9 |
| | 75 | 97.8 | 97.6 | 97.7 | 97.7 | 10.8 | 11.1 | 10.9 | 10.7 | 15.9 | 15.8 | 15.9 | 15.8 |
| | 90 | 100 | 100 | 100 | 100 | 31.6 | 31.3 | 31.2 | 31.2 | 57.1 | 57.6 | 56.9 | 56.4 |
| | 105 | 100 | 100 | 100 | 100 | 93.4 | 93.0 | 93.5 | 93.5 | 99.9 | 99.8 | 99.9 | 99.9 |
| 1200 | 60 | 30.3 | 31.7 | 31.2 | 30.8 | 7.2 | 6.7 | 6.8 | 7.3 | 7.9 | 7.2 | 7.9 | 7.5 |
| | 75 | 98.4 | 98.2 | 98.5 | 98.4 | 11.3 | 11.2 | 11.3 | 11.3 | 15.7 | 16.0 | 15.6 | 15.9 |
| | 90 | 100 | 100 | 100 | 100 | 34.5 | 35.4 | 35.4 | 34.9 | 63.4 | 63.7 | 63.5 | 62.1 |
| | 105 | 100 | 100 | 100 | 100 | 97.5 | 97.3 | 97.6 | 97.5 | 100 | 100 | 100 | 100 |

| | | $T_\gamma/\sqrt{\hat{\sigma}_\gamma}$ | | | | | | | | | | | |
|---|---|---|---|---|---|---|---|---|---|---|---|---|---|
| | | M1 | | | | M2 | | | | M3 | | | |
| $p$ | $\delta$ | F1 | F2 | F3 | F4 | F1 | F2 | F3 | F4 | F1 | F2 | F3 | F4 |
| 200 | 60 | 23.7 | 24.7 | 23.7 | 24.2 | 6.7 | 7.0 | 7.1 | 7.4 | 7.5 | 7.6 | 7.4 | 7.0 |
| | 75 | 79.6 | 79.6 | 79.3 | 79.4 | 8.8 | 9.5 | 9.1 | 9.3 | 11.7 | 11.5 | 11.3 | 11.7 |
| | 90 | 100 | 100 | 100 | 100 | 16.8 | 17.1 | 17.5 | 17.2 | 27.6 | 28.8 | 28.0 | 28.5 |
| | 105 | 100 | 100 | 100 | 100 | 48.5 | 49.1 | 47.9 | 48.6 | 78.4 | 78.8 | 78.0 | 78.2 |
| 400 | 60 | 23.7 | 22.6 | 22.6 | 22.8 | 7.0 | 6.7 | 6.5 | 6.8 | 6.5 | 7.1 | 7.4 | 6.9 |
| | 75 | 84.3 | 84.5 | 83.7 | 83.9 | 9.4 | 8.7 | 8.5 | 9.3 | 11.9 | 12.2 | 11.0 | 11.9 |
| | 90 | 100 | 100 | 100 | 100 | 19.0 | 20.1 | 19.4 | 19.3 | 32.8 | 33.7 | 33.1 | 32.6 |
| | 105 | 100 | 100 | 100 | 100 | 64.3 | 63.8 | 64.3 | 63.8 | 91.5 | 91.0 | 91.8 | 91.2 |
| 800 | 60 | 22.2 | 22.8 | 22.4 | 21.9 | 6.8 | 6.8 | 6.3 | 6.7 | 6.8 | 7.1 | 7.0 | 6.6 |
| | 75 | 88.2 | 88.2 | 88.4 | 88.3 | 9.3 | 9.1 | 9.5 | 9.9 | 12.3 | 12.0 | 11.6 | 12.1 |
| | 90 | 100 | 100 | 100 | 100 | 22.7 | 22.8 | 21.6 | 22.3 | 39.9 | 40.2 | 40.3 | 39.5 |
| | 105 | 100 | 100 | 100 | 100 | 80.0 | 80.4 | 80.2 | 79.9 | 98.3 | 98.3 | 98.2 | 98.4 |
| 1200 | 60 | 22.2 | 21.5 | 22.1 | 21.3 | 6.2 | 6.2 | 6.4 | 6.1 | 6.3 | 6.7 | 7.0 | 6.8 |
| | 75 | 90.4 | 90.6 | 90.4 | 89.9 | 9.2 | 9.1 | 9.6 | 8.8 | 12.0 | 12.0 | 12.1 | 12.0 |
| | 90 | 100 | 100 | 100 | 100 | 25.6 | 24.8 | 25.0 | 24.3 | 43.7 | 43.7 | 43.9 | 43.6 |
| | 105 | 100 | 100 | 100 | 100 | 88.5 | 88.4 | 88.8 | 88.6 | 99.7 | 99.5 | 99.6 | 99.7 |

In our notation (see Section S4.3), $\boldsymbol{X} = (\boldsymbol{X}'_{11}, \boldsymbol{X}'_{12}, \boldsymbol{X}'_{21}, \boldsymbol{X}'_{22}, \boldsymbol{X}'_{31}, \boldsymbol{X}'_{32})'$ represent a complete $N \times p$ data matrix with six sub-matrices, and $\boldsymbol{X}_{ij} = (\boldsymbol{x}_{ij1}, \ldots, \boldsymbol{x}_{ijN_{ij}})'$ is $N_{ij} \times p$ for $i \in \{1,2,3\}$, $j \in \{1,2\}$. In the dataset, we can find $N_{ij} = 4$ observations for $a = 3$ different tissues along with $b = 2$ different feeding statuses. The total sample size is $N = \sum_{i=1}^{3} \sum_{j=1}^{2} N_{ij} = 24$ and all observation vectors have $p = 1,000$ features. Thus, the dataset represents a balanced, high-dimensional, two-way MANOVA experiment with $ab = 6$ independent samples. Furthermore, each observation is modeled as follows:

$$\boldsymbol{x}_{ijk} = \boldsymbol{\eta}_{ij} + \boldsymbol{\varepsilon}_{ijk}, \quad i \in \{1,2,3\}, \quad j \in \{1,2\}, \quad k \in \{1, \ldots, 4\},$$

where $\boldsymbol{\eta}_{ij}$ is the mean for the $(i,j)$-th treatment group; using the decomposition $\boldsymbol{\eta}_{ij} = \boldsymbol{\mu} + \boldsymbol{\alpha}_i + \boldsymbol{\beta}_j + \boldsymbol{\gamma}_{ij}$ provided by (25), $\boldsymbol{\alpha}_i$ represents the effect of the $i$-th type of tissue, $\boldsymbol{\beta}_j$ is the effect of the $j$-th type of feeding status, and $\boldsymbol{\gamma}_{ij}$ is the effect of the interaction between tissue type $i$ and feeding status $j$. The hypotheses of interest can be formulated as follows:

$$\begin{aligned} &H_\alpha : \boldsymbol{\alpha}_i = \mathbf{0}, \quad \forall i \in \{1,2,3\}; \\ &H_\beta : \boldsymbol{\beta}_j = \mathbf{0}, \quad \forall j \in \{1,2\}; \\ &H_\gamma : \boldsymbol{\gamma}_{ij} = \mathbf{0}, \quad \forall i \in \{1,2,3\}, \quad \forall j \in \{1,2\}. \end{aligned}$$

We use the proposed two-way MANOVA test procedures based on the re-scaled $T_\alpha$, $T_\beta$, and $T_\gamma$ from Section S4.3, to test $H_\alpha$, $H_\beta$, and $H_\gamma$, respectively. The observed values of the test statistics are $T_\alpha/\hat{\sigma}_\alpha = 309.78$, $T_\beta/\hat{\sigma}_\alpha = 28.03$, and $T_\gamma/\hat{\sigma}_\gamma = 8.04$, wherein the $p$-value is virtually zero in each case. For all tests, the results provide strong evidence for the rejection of the null hypothesis at any reasonable nominal size, thereby indicating that the marginal effects of the tissue type and feeding status, as well as their combined effects, are highly significant for the variations observed in the DNA gene expression profiles.

## References


[1] Malwane M.A. Ananda and Samaradasa Weerahandi. Two-Way ANOVA with unequal cell frequencies and unequal variances. *Statistica Sinica*, 7(3):631–646, 1997.

[2] Song Xi Chen and Ying-Li Qin. A two-sample test for high-dimensional data with applications to gene-set testing. *Ann. Statist.*, 38(2):808–835, 2010.

[3] Yasunori Fujikoshi, Vladimir V. Ulyanov, and Ryoichi Shimizu. *Multivariate Statistics: High-Dimensional and Large-Sample Approximations.* Wiley Series in Probability and Statistics. John Wiley & Sons, Inc., Hoboken, NJ, 2010.

[4] Yuji Nakai, Hiroko Hashida, Koji Kadota, Michiko Minami, Kentaro Shimizu, Ichiro Matsumoto, Hisanori Kato, and Keiko Abe. Up-regulation of genes related to the ubiquitin-proteasome system in the brown adipose tissue of 24-h-fasted rats. *Bioscience, Biotechnology and Biochemistry*, 72(1):139–148, 2008.

[5] James R. Schott. *Matrix analysis for statistics*. Wiley Series in Probability and Statistics. John Wiley & Sons, Inc., Hoboken, NJ, third edition, 2017.

[6] Muni S. Srivastava. *Methods of Multivariate Statistics*. Wiley Series in Probability and Statistics. Wiley-Interscience [John Wiley & Sons], New York, 2002.

[7] Takayuki Yamada and Tetsuto Himeno. Testing homogeneity of mean vectors under heteroscedasticity in high-dimension. *J. Multivariate Anal.*, 139:7–27, 2015.

[8] Bu Zhou, Jia Guo, and Jin-Ting Zhang. High-dimensional general linear hypothesis testing under heteroscedasticity. *J. Statist. Plann. Inference*, 188:36–54, 2017.
